# Supplementary material for: Structured prior distributions for the covariance matrix in latent factor models
Source: arXiv:2208.07831 ancillary file (2024-06-28)
Supplement: Supplementary file 1 [file supplMat.pdf]

# Supplementary information for *"Structured prior distributions for the covariance matrix in latent factor models"*

Sarah E. Heaps
Durham University, Durham, U.K.
Email: sarah.e.heaps@durham.ac.uk

**Abstract**

Supplementary material contained in this note include derivations of the results used in the paper, complete descriptions of the adaptive Gibbs samplers, and further background and results on the two applications.

## S1 Prior for the identified factor loadings matrix

Section 3 of the main manuscript describes two prior distributions for the parameter-expanded factor loadings matrix $\varLambda \in \mathbb{R}^{p\times k}$: (i) a matrix-normal prior, $\varLambda \sim \mathrm{N}_{p,k}(0, \varPhi, \varPsi)$ and (ii) a matrix-$t$ prior, $\varLambda \sim \mathrm{t}_{p,k}(\varsigma, 0, \breve{\varPhi}, \varPsi)$. An identifiable factor loadings matrix $\tilde{\varLambda} \in \mathbb{R}^{p\times k}$, which satisfies the PLT constraint, can be calculated from $\varLambda$ by taking a LQ decomposition, $\varLambda = \tilde{\varLambda}Q$, in which $Q$ is a $k \times k$ orthogonal matrix. This decomposition will be unique as long as $p \geq k$ and $\varLambda$ is full rank. Therefore, we can, in principle, calculate the prior density induced for the identifiable factor loadings matrix $\tilde{\varLambda}$ by computing the joint density for $(\tilde{\varLambda}, Q)$ and then integrating out $Q$.

Slight modification to Theorem 2.1.13 in Muirhead (2005) yields the Jacobian of the LQ decomposition from $\varLambda$ to $(\tilde{\varLambda}, Q)$ as

$$J(\varLambda \to \tilde{\varLambda}, Q) = \prod_{i=1}^{k} \tilde{\lambda}_{ii}^{k-i} (Q\ dQ^{\mathrm{T}})$$

where $(Q\ dQ^{\mathrm{T}})$ is the Haar measure on the orthogonal group. Therefore, given a matrix normal or matrix $t$-density $p_{\Lambda}(\cdot)$ for the random matrix $\varLambda$, the joint prior for $(\tilde{\varLambda}, Q)$ has the form

$$p_{\Lambda}(\tilde{\varLambda}Q) \prod_{i=1}^{k} \tilde{\lambda}_{ii}^{k-i} (d\tilde{\varLambda})(Q\ dQ^{\mathrm{T}}). \tag{S1}$$

Under certain conditions, a matrix normal distribution for $\varLambda$ yields a prior for $\tilde{\varLambda}$ that can be described using standard distributional families. The remainder of this section focuses on this specific special case.

If a random matrix $\varLambda$ has a matrix normal distribution, $\varLambda \sim \mathrm{N}_{p,k}(0, \varPhi, \varPsi)$, then its probability density function is

$$p(\varLambda) = \frac{1}{(2\pi)^{pk} |\varPsi|^{p/2} |\varPhi|^{k/2}} \exp\left\{ -\frac{1}{2} \mathrm{tr}\left( \varPhi^{-1} \varLambda \varPsi^{-1} \varLambda^{\mathrm{T}} \right) \right\}, \quad \varLambda \in \mathbb{R}^{p\times k}.$$

Substituting this density into (S1) yields

$$\frac{1}{(2\pi)^{pk} |\varPsi|^{p/2} |\varPhi|^{k/2}} \exp\left\{ -\frac{1}{2} \mathrm{tr}\left( \varPhi^{-1} \tilde{\varLambda} Q \varPsi^{-1} Q^{\mathrm{T}} \tilde{\varLambda}^{\mathrm{T}} \right) \right\} \prod_{i=1}^{k} \tilde{\lambda}_{ii}^{k-i} (d\tilde{\varLambda})(Q\ dQ^{\mathrm{T}}). \tag{S2}$$

In the general case, $\tilde{\Lambda}$ and $Q$ are not independent *a priori*. Though the conditional distribution of $Q$ given $\tilde{\Lambda}$ is a matrix-variate Bingham distribution (Hoff, 2009), its normalising constant is not computationally tractable and so the marginal distribution of $\tilde{\Lambda}$ cannot, in general, be obtained in closed form. However, in the special case when $\Psi = \psi I_k$, the joint and marginal distributions of $\tilde{\Lambda}$ and $Q$ can be derived explicitly. To this end, let $\tilde{\boldsymbol{\lambda}}_{(i)j} = (\tilde{\lambda}_{ij}, \dots, \tilde{\lambda}_{pj})^{\mathrm{T}}$ denote the elements in rows $i$ to $p$ and column $j$ of $\tilde{\Lambda}$, and denote by $\Xi_{(i)}$ the submatrix of $\Xi = \Phi^{-1}$ spanning rows $i$ to $p$ and columns $i$ to $p$, partitioned as

$$\Xi_{(i)} = \begin{pmatrix} \xi_{ii} & \boldsymbol{\xi}_{(i+1)i}^{\mathrm{T}} \\ \boldsymbol{\xi}_{(i+1)i} & \Xi_{(i+1)} \end{pmatrix} \tag{S3}$$

where $\boldsymbol{\xi}_{(i+1)i} = (\xi_{i+1,i}, \dots, \xi_{pi})^{\mathrm{T}}$. We then have the following Theorem.

**Theorem 1.** *Let $\Lambda = \tilde{\Lambda} Q$ be the LQ decomposition of the $p \times k$ random matrix $\Lambda \sim \mathrm{N}_{p,k}(0, \Phi, \psi I_k)$ where $p \geq k$. Then the lower triangular matrix with positive diagonal elements $\tilde{\Lambda}$ and the orthogonal matrix $Q$ are independent. Moreover, the matrix $Q$ is distributed according to the Haar measure over the orthogonal group while $\tilde{\Lambda}$ is distributed such that $\tilde{\boldsymbol{\lambda}}_{(1)1}, \dots, \tilde{\boldsymbol{\lambda}}_{(k)k}$ are independent across columns with within-column distribution*

$$\tilde{\lambda}_{ii}^2 \sim \mathrm{Gam}\left\{ \frac{k-i+1}{2},\ \frac{1}{2\psi}\left( \xi_{ii} - \boldsymbol{\xi}_{(i+1)i}^{\mathrm{T}} \Xi_{(i+1)}^{-1} \boldsymbol{\xi}_{(i+1)i} \right) \right\} \tag{S4}$$

*and*

$$\tilde{\boldsymbol{\lambda}}_{(i+1)i} | \tilde{\lambda}_{ii} \sim \mathrm{N}_{p-i}\left( -\tilde{\lambda}_{ii} \Xi_{(i+1)}^{-1} \boldsymbol{\xi}_{(i+1)i},\ \psi \Xi_{(i+1)}^{-1} \right) \tag{S5}$$

*for column $i = 1, \dots, k$.*

*Proof.* Substituting $\Psi = \psi I_k$ and $\Phi^{-1} = \Xi$ into (S2) and applying the cyclic property of the trace operator yields

$$\frac{1}{(2\pi)^{pk} |\Phi|^{k/2} \psi^{pk/2}} \exp\left\{ -\frac{1}{2\psi} \mathrm{tr}\left( \tilde{\Lambda}^{\mathrm{T}} \Xi \tilde{\Lambda} \right) \right\} \prod_{i=1}^{k} \tilde{\lambda}_{ii}^{k-i} (d\tilde{\Lambda})(Q\ dQ^{\mathrm{T}}),$$

from which it is clear that $\tilde{\Lambda}$ and $Q$ are independent *a priori*, the distribution of $Q$ is a (normalized) Haar measure, and the density of $\tilde{\Lambda}$ is given by

$$p_{\tilde{\Lambda}}(\tilde{\Lambda}) \propto \exp\left\{ -\frac{1}{2\psi} \mathrm{tr}\left( \tilde{\Lambda}^{\mathrm{T}} \Xi \tilde{\Lambda} \right) \right\} \prod_{i=1}^{k} \tilde{\lambda}_{ii}^{k-i}. \tag{S6}$$

Noting that $\tilde{\boldsymbol{\lambda}}_{(1)i}^{\mathrm{T}} = (\mathbf{0}^{\mathrm{T}}, \tilde{\boldsymbol{\lambda}}_{(i)i}^{\mathrm{T}})$, the required trace in (S6) is clearly

$$\mathrm{tr}\left( \tilde{\Lambda}^{\mathrm{T}} \Xi \tilde{\Lambda} \right) = \sum_{i=1}^{k} \tilde{\boldsymbol{\lambda}}_{(1)i}^{\mathrm{T}} \Xi \tilde{\boldsymbol{\lambda}}_{(1)i} = \sum_{i=1}^{k} \begin{pmatrix} \mathbf{0}^{\mathrm{T}} & \tilde{\boldsymbol{\lambda}}_{(i)i}^{\mathrm{T}} \end{pmatrix} \begin{pmatrix} * & * \\ * & \Xi_{(i)} \end{pmatrix} \begin{pmatrix} \mathbf{0} \\ \tilde{\boldsymbol{\lambda}}_{(i)i} \end{pmatrix} = \sum_{i=1}^{k} \tilde{\boldsymbol{\lambda}}_{(i)i}^{\mathrm{T}} \Xi_{(i)} \tilde{\boldsymbol{\lambda}}_{(i)i}.$$

It follows that (S6) can be written as

$$p_{\tilde{\Lambda}}(\tilde{\Lambda}) \propto \prod_{i=1}^{k} \left\{ \exp\left( -\frac{1}{2\psi} \tilde{\boldsymbol{\lambda}}_{(i)i}^{\mathrm{T}} \Xi_{(i)} \tilde{\boldsymbol{\lambda}}_{(i)i} \right) \tilde{\lambda}_{ii}^{k-i} \right\}.$$

The factorization over the columns of $\tilde{\Lambda}$ implies immediately that $\tilde{\boldsymbol{\lambda}}_{(1)1}, \dots, \tilde{\boldsymbol{\lambda}}_{(k)k}$ are independent. Partitioning $\Xi_{(i)}$ as in (S3), the density of $\tilde{\boldsymbol{\lambda}}_{(i)i}^{\mathrm{T}} = (\tilde{\lambda}_{ii}, \tilde{\boldsymbol{\lambda}}_{(i+1)i}^{\mathrm{T}})$ is then proportional to

$$\begin{aligned} p(\tilde{\boldsymbol{\lambda}}_{(i)i}) &\propto \exp\left( -\frac{1}{2\psi} \tilde{\boldsymbol{\lambda}}_{(i)i}^{\mathrm{T}} \Xi_{(i)} \tilde{\boldsymbol{\lambda}}_{(i)i} \right) \tilde{\lambda}_{ii}^{k-i} \\ &= \exp\left\{ -\frac{1}{2\psi} \left( \tilde{\boldsymbol{\lambda}}_{(i+1)i} + \tilde{\lambda}_{ii} \Xi_{(i+1)}^{-1} \boldsymbol{\xi}_{(i+1)i} \right)^{\mathrm{T}} \Xi_{(i+1)} \left( \tilde{\boldsymbol{\lambda}}_{(i+1)i} + \tilde{\lambda}_{ii} \Xi_{(i+1)}^{-1} \boldsymbol{\xi}_{(i+1)i} \right) \right\} \\ &\quad \times \exp\left\{ -\frac{1}{2\psi} \left( \xi_{ii} - \boldsymbol{\xi}_{(i+1)i}^{\mathrm{T}} \Xi_{(i+1)}^{-1} \boldsymbol{\xi}_{(i+1)i} \right) \tilde{\lambda}_{ii}^2 \right\} \tilde{\lambda}_{ii}^{k-i}. \end{aligned} \tag{S7}$$

We now need to introduce a second change of variables

$$\tilde{\lambda}_{ii} = \tilde{\lambda}_i^{*\,1/2}$$

so that

$$\frac{d\tilde{\lambda}_{ii}}{d\tilde{\lambda}_i^*} = 2^{-1}\tilde{\lambda}_i^{*\,-1/2}$$

and then (S7) becomes

$$p(\tilde{\lambda}_i^*, \tilde{\boldsymbol{\lambda}}_{(i+1)i}) \propto \exp\left\{-\frac{1}{2\psi}\left(\tilde{\boldsymbol{\lambda}}_{(i+1)i} + \tilde{\lambda}_i^{*\,1/2}\varXi_{(i+1)}^{-1}\boldsymbol{\xi}_{(i+1)i}\right)^{\mathrm{T}}\varXi_{(i+1)}\left(\tilde{\boldsymbol{\lambda}}_{(i+1)i} + \tilde{\lambda}_i^{*\,1/2}\varXi_{(i+1)}^{-1}\boldsymbol{\xi}_{(i+1)i}\right)\right\}$$
$$\times \exp\left\{-\frac{1}{2\psi}\left(\xi_{ii} - \boldsymbol{\xi}_{(i+1)i}^{\mathrm{T}}\varXi_{(i+1)}^{-1}\boldsymbol{\xi}_{(i+1)i}\right)\tilde{\lambda}_i^*\right\}\tilde{\lambda}_i^{*\,(k-i-1)/2}.$$

It follows that

$$\tilde{\lambda}_i^* \equiv \tilde{\lambda}_{ii}^2 \sim \mathrm{Gam}\left(\frac{k-i+1}{2},\ \frac{1}{2\psi}\left(\xi_{ii} - \boldsymbol{\xi}_{(i+1)i}^{\mathrm{T}}\varXi_{(i+1)}^{-1}\boldsymbol{\xi}_{(i+1)i}\right)\right),$$

and

$$\tilde{\boldsymbol{\lambda}}_{(i+1)i}|\tilde{\lambda}_i^* \sim \mathrm{N}_{p-i}\left(-\tilde{\lambda}_i^{*\,1/2}\varXi_{(i+1)}^{-1}\boldsymbol{\xi}_{(i+1)i},\ \psi\varXi_{(i+1)}^{-1}\right),$$

for $i = 1, \ldots, k$ as required. □

In the special case when $\varPhi = I_p$ in addition to $\varPsi = \psi I_k$, we obtain the following corollary to Theorem 1, which is equivalent to Theorem 2.1 in Leung and Drton (2016).

**Corollary 1.1.** *Let $\varLambda = \tilde{\varLambda}Q$ be the LQ decomposition of the $p \times k$ random matrix $\varLambda \sim \mathrm{N}_{p,k}(0, I_p, \psi I_k)$ where $p \geq k$. Then the lower triangular matrix with positive diagonal elements $\tilde{\varLambda}$ and the orthogonal matrix $Q$ are independent, the matrix $Q$ is distributed according to the Haar measure over the orthogonal group, while the non-zero elements in $\tilde{\varLambda}$ are independent and, for $i = 1, \ldots, k$, distributed such that*

$$\tilde{\lambda}_{ii}^2 \sim \mathrm{Gam}\left(\frac{k-i+1}{2},\ \frac{1}{2\psi}\right)$$

*and*

$$\tilde{\lambda}_{ij} \sim \mathrm{N}(0, \psi), \quad j = 1, \ldots, i-1.$$

*Proof.* Set $\varXi = I_p$ and then $\varXi_{(i)} = I_{p-i+1}$, $\xi_{ii} = 1$ and $\boldsymbol{\xi}_{(i+1)i} = \mathbf{0}$. Substituting these expressions into (S4) and (S5) yields the desired result. □

# S2 Derivation of moments for the shared variation

Sections 3.2–3.4 of the manuscript present the means, variances and covariances between elements $\delta_{ij}$ in the $p \times p$ shared variation matrix $\varDelta = \varLambda\varLambda^{\mathrm{T}}$ under the matrix normal and matrix-$t$ priors for the factor loadings matrix $\varLambda$. In this section, the derivations of those results are presented.

## S2.1 Prior based on matrix normal distribution

The calculations that follow make use of numerous numbered Theorems from Chapters 2, 3 and 4 of Gupta and Nagar (2000) (hereafter GN), as indicated. From GN Theorem 2.3.5(ii), it follows that the required expectation is given by

$$E(\varDelta) = E(\varLambda\varLambda^{\mathrm{T}}) = \mathrm{tr}(\varPsi)\varPhi. \tag{S8}$$

The general form for the covariance between $\delta_{ij}$ and $\delta_{k\ell}$ was given in equation (3) of the manuscript. For its calculation, we first need to compute $E(\varLambda\varLambda^{\mathrm{T}}\boldsymbol{e}_i\boldsymbol{e}_k^{\mathrm{T}}\varLambda\varLambda^{\mathrm{T}})$. This follows from GN Theorem 2.3.8(v) as

$$E(\varLambda\varLambda^{\mathrm{T}}\boldsymbol{e}_i\boldsymbol{e}_k^{\mathrm{T}}\varLambda\varLambda^{\mathrm{T}}) = \mathrm{tr}(\varPsi^2)\phi_{ik}\varPhi + \mathrm{tr}(\varPsi)^2\boldsymbol{\phi}^{(i)}\boldsymbol{\phi}_k^{\mathrm{T}} + \mathrm{tr}(\varPsi^2)\boldsymbol{\phi}^{(k)}\boldsymbol{\phi}_i^{\mathrm{T}}$$

in which $\boldsymbol{\phi}^{(i)}$ and $\boldsymbol{\phi}_i^{\mathrm{T}}$ denote the $i$th column and row of $\varPhi$, respectively. Pre-multiplication by $\boldsymbol{e}_j^{\mathrm{T}}$ and post-multiplication by $\boldsymbol{e}_\ell$ then yields

$$\boldsymbol{e}_j^{\mathrm{T}}E(\varLambda\varLambda^{\mathrm{T}}\boldsymbol{e}_i\boldsymbol{e}_k^{\mathrm{T}}\varLambda\varLambda^{\mathrm{T}})\boldsymbol{e}_\ell = \mathrm{tr}(\varPsi^2)\phi_{ik}\phi_{j\ell} + \mathrm{tr}(\varPsi)^2\phi_{ij}\phi_{k\ell} + \mathrm{tr}(\varPsi^2)\phi_{i\ell}\phi_{jk}.$$

Using (S8), the product of the second order moments in (3) is given by

$$\boldsymbol{e}_j^{\mathrm{T}}E(\varLambda\varLambda^{\mathrm{T}})\boldsymbol{e}_i\boldsymbol{e}_k^{\mathrm{T}}E(\varLambda\varLambda^{\mathrm{T}})\boldsymbol{e}_\ell = \mathrm{tr}(\varPsi)^2\phi_{ij}\phi_{k\ell}.$$

The covariance between $\delta_{ij}$ and $\delta_{k\ell}$ is therefore

$$\mathrm{Cov}(\delta_{ij}, \delta_{k\ell}) = \mathrm{tr}(\varPsi^2)(\phi_{ik}\phi_{j\ell} + \phi_{i\ell}\phi_{jk}).$$

In the special case where $i = k$ and $j = \ell$, the variance of $\delta_{ij}$ is given by

$$\mathrm{Var}(\delta_{ij}) = \mathrm{tr}(\varPsi^2)(\phi_{ii}\phi_{jj} + \phi_{ij}^2).$$

## S2.2 Prior based on matrix-$t$ distribution

The calculations in this section rely on the representation of a matrix-$t$ random variable expressed through (6) of the manuscript, from which it can be deduced that $\varLambda | S \sim \mathrm{N}_{p,k}(M, S^{-1}, \varPsi)$. From GN Theorem 4.3.2(ii), it follows that the required expectation is given by

$$E(\varDelta) = E(\varLambda\varLambda^{\mathrm{T}}) = \frac{\mathrm{tr}(\varPsi)}{\varsigma - 2}\breve{\varPhi} \tag{S9}$$

for $\varsigma > 2$.

In the calculation of the covariances, using the Law of Total Expectation we have

$$\begin{aligned}
&E(\varLambda\varLambda^{\mathrm{T}}\boldsymbol{e}_i\boldsymbol{e}_k^{\mathrm{T}}\varLambda\varLambda^{\mathrm{T}}) \\
&\quad = E_S\{E_{\Lambda|S}(\varLambda\varLambda^{\mathrm{T}}\boldsymbol{e}_i\boldsymbol{e}_k^{\mathrm{T}}\varLambda\varLambda^{\mathrm{T}})\} \\
&\quad = E_S\{\mathrm{tr}(\varPsi^2)\mathrm{tr}(\boldsymbol{e}_i\boldsymbol{e}_k^{\mathrm{T}}S^{-1})S^{-1} + \mathrm{tr}(\varPsi)^2S^{-1}\boldsymbol{e}_i\boldsymbol{e}_k^{\mathrm{T}}S^{-1} + \mathrm{tr}(\varPsi^2)S^{-1}\boldsymbol{e}_k\boldsymbol{e}_i^{\mathrm{T}}S^{-1}\} \\
&\quad = \mathrm{tr}(\varPsi^2)E_S\{\mathrm{tr}(\boldsymbol{e}_i\boldsymbol{e}_k^{\mathrm{T}}S^{-1})S^{-1}\} + \mathrm{tr}(\varPsi)^2E_S(S^{-1}\boldsymbol{e}_i\boldsymbol{e}_k^{\mathrm{T}}S^{-1}) + \mathrm{tr}(\varPsi^2)E_S(S^{-1}\boldsymbol{e}_k\boldsymbol{e}_i^{\mathrm{T}}S^{-1}).
\end{aligned} \tag{S10}$$

Now, if $\varsigma > 4$ we define

$$c_2 = \{(\varsigma - 1)(\varsigma - 2)(\varsigma - 4)\}^{-1}, \qquad c_1 = (\varsigma - 3)c_2.$$

Using GN Theorem 3.3.18(ii), the first expectation on the right-hand-side of (S10) can be simplified as follows

$$\begin{aligned}
E_S\{\mathrm{tr}(\boldsymbol{e}_i\boldsymbol{e}_k^{\mathrm{T}}S^{-1})S^{-1}\} &= c_1\mathrm{tr}(\boldsymbol{e}_i\boldsymbol{e}_k^{\mathrm{T}}\breve{\varPhi})\breve{\varPhi} + c_2(\breve{\varPhi}\boldsymbol{e}_k\boldsymbol{e}_i^{\mathrm{T}}\breve{\varPhi} + \breve{\varPhi}\boldsymbol{e}_i\boldsymbol{e}_k^{\mathrm{T}}\breve{\varPhi}) \\
&= c_1\breve{\phi}_{ik}\breve{\varPhi} + c_2(\breve{\boldsymbol{\phi}}^{(k)}\breve{\boldsymbol{\phi}}_i^{\mathrm{T}} + \breve{\boldsymbol{\phi}}^{(i)}\breve{\boldsymbol{\phi}}_k^{\mathrm{T}}).
\end{aligned}$$

Using GN Theorem 3.3.18(i), the second expectation can be written

$$\begin{aligned}
E_S(S^{-1}\boldsymbol{e}_i\boldsymbol{e}_k^{\mathrm{T}}S^{-1}) &= c_1\breve{\varPhi}\boldsymbol{e}_i\boldsymbol{e}_k^{\mathrm{T}}\breve{\varPhi} + c_2\left\{\breve{\varPhi}\boldsymbol{e}_k\boldsymbol{e}_i^{\mathrm{T}}\breve{\varPhi} + \mathrm{tr}(\boldsymbol{e}_i\boldsymbol{e}_k^{\mathrm{T}}\breve{\varPhi})\breve{\varPhi}\right\} \\
&= c_1\breve{\boldsymbol{\phi}}^{(i)}\breve{\boldsymbol{\phi}}_k^{\mathrm{T}} + c_2(\breve{\boldsymbol{\phi}}^{(k)}\breve{\boldsymbol{\phi}}_i^{\mathrm{T}} + \breve{\phi}_{ik}\breve{\varPhi}),
\end{aligned}$$

and, analogously, the third expectation becomes

$$E_S(S^{-1}\boldsymbol{e}_k\boldsymbol{e}_i^{\mathrm{T}}S^{-1}) = c_1\breve{\boldsymbol{\phi}}^{(k)}\breve{\boldsymbol{\phi}}_i^{\mathrm{T}} + c_2(\breve{\boldsymbol{\phi}}^{(i)}\breve{\boldsymbol{\phi}}_k^{\mathrm{T}} + \breve{\phi}_{ik}\breve{\Phi}).$$

Substituting these expressions back into (S10) gives

$$\begin{aligned} E(\Lambda\Lambda^{\mathrm{T}}\boldsymbol{e}_i\boldsymbol{e}_k^{\mathrm{T}}\Lambda\Lambda^{\mathrm{T}}) = &\left\{\mathrm{tr}(\Psi^2)(c_1+c_2) + \mathrm{tr}(\Psi)^2c_2\right\}(\breve{\phi}_{ik}\breve{\Phi} + \breve{\boldsymbol{\phi}}^{(k)}\breve{\boldsymbol{\phi}}_i^{\mathrm{T}}) \\ &+ \left\{2\mathrm{tr}(\Psi^2)c_2 + \mathrm{tr}(\Psi)^2c_1\right\}\breve{\boldsymbol{\phi}}^{(i)}\breve{\boldsymbol{\phi}}_k^{\mathrm{T}}. \end{aligned}$$

Pre-multiplication by $\boldsymbol{e}_j^{\mathrm{T}}$ and post-multiplication by $\boldsymbol{e}_\ell$ then yields

$$\begin{aligned} &\boldsymbol{e}_j^{\mathrm{T}}E(\Lambda\Lambda^{\mathrm{T}}\boldsymbol{e}_i\boldsymbol{e}_k^{\mathrm{T}}\Lambda\Lambda^{\mathrm{T}})\boldsymbol{e}_\ell \\ &\quad = \left\{\mathrm{tr}(\Psi^2)(c_1+c_2) + \mathrm{tr}(\Psi)^2c_2\right\}(\breve{\phi}_{i\ell}\breve{\phi}_{jk} + \breve{\phi}_{ik}\breve{\phi}_{j\ell}) + \left\{2\mathrm{tr}(\Psi^2)c_2 + \mathrm{tr}(\Psi)^2c_1\right\}\breve{\phi}_{ij}\breve{\phi}_{k\ell} \\ &\quad = c_2\left\{\mathrm{tr}(\Psi^2)(\varsigma-2) + \mathrm{tr}(\Psi)^2\right\}(\breve{\phi}_{i\ell}\breve{\phi}_{jk} + \breve{\phi}_{ik}\breve{\phi}_{j\ell}) + c_2\left\{2\mathrm{tr}(\Psi^2) + \mathrm{tr}(\Psi)^2(\varsigma-3)\right\}\breve{\phi}_{ij}\breve{\phi}_{k\ell}. \end{aligned}$$

Using (S9), the product of the second order moments in (3) is given by

$$\boldsymbol{e}_j^{\mathrm{T}}E(\Lambda\Lambda^{\mathrm{T}})\boldsymbol{e}_i\boldsymbol{e}_k^{\mathrm{T}}E(\Lambda\Lambda^{\mathrm{T}})\boldsymbol{e}_\ell = \frac{\mathrm{tr}(\Psi)^2}{(\varsigma-2)^2}\breve{\phi}_{ij}\breve{\phi}_{k\ell}.$$

The covariance between $\delta_{ij}$ and $\delta_{k\ell}$ is therefore

$$\mathrm{Cov}(\delta_{ij},\delta_{k\ell}) = c_3\left\{\mathrm{tr}(\Psi)^2 + (\varsigma-2)\mathrm{tr}(\Psi^2)\right\}\left\{2\breve{\phi}_{ij}\breve{\phi}_{k\ell} + (\varsigma-2)(\breve{\phi}_{ik}\breve{\phi}_{j\ell} + \breve{\phi}_{i\ell}\breve{\phi}_{jk})\right\}$$

where

$$c_3 = c_2(\varsigma-2)^{-1} = \left\{(\varsigma-1)(\varsigma-2)^2(\varsigma-4)\right\}^{-1}.$$

In the special case where $i=k$ and $j=\ell$, the variance of $\delta_{ij}$ is given by

$$\mathrm{Var}(\delta_{ij}) = c_3\left\{\mathrm{tr}(\Psi)^2 + (\varsigma-2)\mathrm{tr}(\Psi^2)\right\}\left\{\varsigma\breve{\phi}_{ij}^2 + (\varsigma-2)\breve{\phi}_{ii}\breve{\phi}_{jj}\right\}.$$

For parameter interpretation and for the derivation of the results in the next section, it is convenient to reparameterize the distribution for $\Lambda$ and therefore $\Delta$ in terms of $\Phi = \breve{\Phi}/(\varsigma-2)$. The mean then reduces to

$$E(\Delta) = E_\Lambda(\Lambda\Lambda^{\mathrm{T}}) = \mathrm{tr}(\Psi)\Phi, \tag{S11}$$

and the variances and covariances become

$$\mathrm{Cov}(\delta_{ij},\delta_{k\ell}) = \frac{\left\{\mathrm{tr}(\Psi)^2 + (\varsigma-2)\mathrm{tr}(\Psi^2)\right\}\left\{2\phi_{ij}\phi_{k\ell} + (\varsigma-2)(\phi_{ik}\phi_{j\ell} + \phi_{i\ell}\phi_{jk})\right\}}{(\varsigma-1)(\varsigma-4)},$$

and

$$\mathrm{Var}(\delta_{ij}) = \frac{\left\{\mathrm{tr}(\Psi)^2 + (\varsigma-2)\mathrm{tr}(\Psi^2)\right\}\left\{\varsigma\phi_{ij}^2 + (\varsigma-2)\phi_{ii}\phi_{jj}\right\}}{(\varsigma-1)(\varsigma-4)}. \tag{S12}$$

We note that the mean in (S11) now has exactly the same form as that obtained under the matrix normal prior. More significantly, it will be straightforward to study the effects of varying the degree of freedom parameter $\varsigma$ on the variances and covariances while keeping the mean constant.

# S3 Bounding the variance under the matrix-$t$ prior

The Frobenius inner product of two matrices $A \in \mathbb{R}^{n\times m}$ and $B \in \mathbb{R}^{n\times m}$ can be defined as

$$\langle A, B\rangle_F = \mathrm{tr}(A^{\mathrm{T}}B). \tag{S13}$$

We can therefore apply the Cauchy-Schwartz inequality with $A = \mathit{\Psi}$ and $B = I_k$ which yields $\mathrm{tr}(\mathit{\Psi})^2 \le k\mathrm{tr}(\mathit{\Psi}^2)$. Similarly, the norm induced by (S13) – the Frobenius norm – of $A \in \mathbb{R}^{n\times m}$ is defined by

$$\|A\|_F = \sqrt{\mathrm{tr}(A^{\mathrm{T}}A)}.$$

The Frobenius norm possesses the submultiplicative property (see, for example Banerjee and Roy, 2014, Chapter 15). This means that for $A \in \mathbb{R}^{n\times m}$ and $B \in \mathbb{R}^{m\times p}$ we have

$$\|AB\|_F \le \|A\|_F\|B\|_F.$$

We can therefore take $A = \mathit{\Psi}^{1/2}$ and $B = \mathit{\Psi}^{1/2}$ and square each side to give $\mathrm{tr}(\mathit{\Psi}^2) \le \mathrm{tr}(\mathit{\Psi})^2$. Altogether, this implies

$$\frac{1}{k}\mathrm{tr}(\mathit{\Psi})^2 \le \mathrm{tr}(\mathit{\Psi}^2) \le \mathrm{tr}(\mathit{\Psi})^2,$$

and so we can bound the left-hand term in the numerator of the variance in (S12) between

$$\mathrm{tr}(\mathit{\Psi})^2(\varsigma + k - 2)/k \le \mathrm{tr}(\mathit{\Psi})^2 + (\varsigma - 2)\mathrm{tr}(\mathit{\Psi}^2) \le \mathrm{tr}(\mathit{\Psi})^2(\varsigma - 1). \tag{S14}$$

Now, taking $m_{ij} = E(\delta_{ij}) = \mathrm{tr}(\Psi)\phi_{ij}$ in (S12) gives

$$\mathrm{Var}(\delta_{ij}) = \frac{\left\{\mathrm{tr}(\mathit{\Psi})^2 + (\varsigma - 2)\mathrm{tr}(\mathit{\Psi}^2)\right\}\left\{\varsigma m_{ij}^2 + (\varsigma - 2)m_{ii}m_{jj}\right\}}{\mathrm{tr}(\Psi)^2(\varsigma - 1)(\varsigma - 4)}$$

and so we can use (S14) to bound the variance between

$$\frac{(\varsigma + k - 2)\{\varsigma m_{ij}^2 + (\varsigma - 2)m_{ii}m_{jj}\}}{k(\varsigma - 1)(\varsigma - 4)} \le \mathrm{Var}(\delta_{ij}) \le \frac{\varsigma m_{ij}^2 + (\varsigma - 2)m_{ii}m_{jj}}{\varsigma - 4}.$$

For fixed values of the means $m_{ij}$, the lower and upper bounds are rational functions in $\varsigma$, each of which is defined and positive for all $\varsigma > 4$. The lower limit approaches the horizontal asymptote $(m_{ij}^2 + m_{ii}m_{jj})/k$ as $\varsigma \to \infty$ whilst the upper limit approaches the horizontal asymptote $(m_{ij}^2 + m_{ii}m_{jj})$. Moreover, $\varsigma = 4$ is a vertical asymptote. This means that the variance $\mathrm{Var}(\delta_{ij})$ is bound between two functions that are finite as $\varsigma \to \infty$ whilst becoming infinite as $\varsigma$ tends to 4 from above. It follows that we can keep the mean constant whilst using the degree of freedom parameter $\varsigma$ to control the variance.

# S4 Markov chain Monte Carlo sampling

## S4.1 Gibbs samplers for static factor models

### S4.1.1 Gibbs sampler with fixed level of truncation

Consider the (static) factor model. Suppose that the matrix normal prior from Section 3.3 has been chosen for $\mathit{\Lambda}$ and that we have completed our prior specification by assuming the idiosyncratic variances are independent and such that $\sigma_j^{-1} \sim \mathrm{Gam}(a_\sigma, b_\sigma)$ for $j = 1, \dots, p$ and that $\boldsymbol{\mu} \sim \mathrm{N}(\boldsymbol{m}_\mu, V_\mu)$. Given a fixed level of truncation $H$, one iteration of the non-adaptive Gibbs sampler involves a sweep through the following steps:

1. For $i = 1, \dots, n$ sample

$$\boldsymbol{\eta}_i | \dots \sim \mathrm{N}_H\left\{(I_H + \mathit{\Lambda}^{\mathrm{T}}\mathit{\Sigma}^{-1}\mathit{\Lambda})^{-1}\mathit{\Lambda}^{\mathrm{T}}\mathit{\Sigma}^{-1}(\boldsymbol{y}_i - \boldsymbol{\mu}),\, (I_H + \mathit{\Lambda}^{\mathrm{T}}\mathit{\Sigma}^{-1}\mathit{\Lambda})^{-1}\right\}.$$

2. Sample $\mathrm{vec}(\Lambda)|\ldots \sim \mathrm{N}_{pH}(\boldsymbol{c}, D^{-1})$ where

$$D = (E^{\mathrm{T}}E \otimes \Sigma^{-1}) + (\Psi \otimes \Phi)^{-1}$$

and

$$\boldsymbol{c} = D^{-1}(E^{\mathrm{T}} \otimes \Sigma^{-1})\mathrm{vec}\{Y - (\mathbf{1}_n \otimes \boldsymbol{\mu}^{\mathrm{T}})\}$$

where $Y$ is a $n \times p$ matrix whose $i$th row is $\boldsymbol{y}_i^{\mathrm{T}}$ and $E$ is a $n \times H$ matrix whose $i$th row is $\boldsymbol{\eta}_i^{\mathrm{T}}$.

3. For $j = 1, \ldots, p$, sample

$$\sigma_j^{-1}|\ldots \mathrm{Gam}\left\{a_\sigma + \frac{n}{2}\,,\, b_\sigma + \frac{1}{2}\sum_{i=1}^{n}(y_{ij} - \mu_j - \boldsymbol{\lambda}_j^{\mathrm{T}}\boldsymbol{\eta}_i)^2\right\}$$

where $\boldsymbol{\lambda}_j^{\mathrm{T}}$ is row $j$ of $\Lambda$.

4. Sample

$$\boldsymbol{\mu}|\ldots \sim \mathrm{N}_p\left\{(P_\mu + n\Sigma^{-1})(P_\mu \boldsymbol{m}_\mu + n\Sigma^{-1}\bar{\boldsymbol{y}}_\eta)\,,\,(P_\mu + n\Sigma^{-1})^{-1}\right\}$$

where $\bar{\boldsymbol{y}}_\eta$ is the sample mean vector of $Y - E\Lambda^{\mathrm{T}}$.

5. Update any correlation parameters, $\boldsymbol{\vartheta}$, in $\Phi$ from

$$\pi(\boldsymbol{\vartheta}|\ldots) \propto \pi(\boldsymbol{\vartheta})\pi(\Lambda|\Phi, \Psi)$$

using a Metropolis-Hastings step.

6. Sample

$$\varrho_1|\ldots \sim \mathrm{Gam}\left(a_1 + \frac{nH}{2}\,,\, 1 + \frac{1}{2}\sum_{h=1}^{H} g_h^{(1)}\boldsymbol{\lambda}^{(h)\,\mathrm{T}}\Phi^{-1}\boldsymbol{\lambda}^{(h)}\right)$$

and then, for $j = 2, \ldots, H$, sample

$$\varrho_j|\ldots \sim \mathrm{Gam}\left(a_2 + \frac{n}{2}(H - j + 1)\,,\, 1 + \frac{1}{2}\sum_{h=j}^{H} g_h^{(j)}\boldsymbol{\lambda}^{(h)\,\mathrm{T}}\Phi^{-1}\boldsymbol{\lambda}^{(h)}\right)$$

where $\boldsymbol{\lambda}^{(h)}$ denotes column $h$ of $\Lambda$ and $g_h^{(j)} = \prod_{\ell=1,\ell\neq j}^{h} \varrho_\ell$ for $j = 1, \ldots, H$.

If, instead, we have chosen a matrix-$t$ prior for $\Lambda$ with unknown degree of freedom parameter $\varsigma$, we substitute $S^{-1}$ in place of $\Phi$ in steps 2 and 6, replace step 5 with

5. Update any correlation parameters, $\boldsymbol{\vartheta}$, in $\breve{\Phi}$ from

$$\pi(\boldsymbol{\vartheta}|\ldots) \propto \pi(\boldsymbol{\vartheta})\pi(S|\varsigma, \breve{\Phi}),$$

where $S|\varsigma, \breve{\Phi} \sim \mathrm{W}_p(\varsigma + p - 1, \breve{\Phi}^{-1})$, using a Metropolis-Hastings step.

We then add the following joint Metropolis-Hastings update between steps 4 and 5

4.5. Update $(S, \varsigma)$ jointly by simulating $\varsigma^*$ from a proposal distribution with density $q(\varsigma^*|\varsigma)$, for example a lognormal distribution with location parameter $\log\varsigma$, and then proposing $S^*$ from its full conditional distribution given $\varsigma^*$:

$$S^*|\varsigma^*, \Lambda, \breve{\Phi}, \Psi \sim \mathrm{W}_p\left\{H + p + \varsigma^* - 1\,,\,(\Lambda\Psi^{-1}\Lambda^{\mathrm{T}} + \breve{\Phi})^{-1}\right\}.$$

In the acceptance probability $\min\{1, A\}$ of the proposal, $A$ simplifies to

$$\begin{aligned} A &= \frac{q_1(\varsigma|\varsigma^*)\pi(S|\varsigma, \Lambda, \breve{\Phi}, \Psi)}{q_1(\varsigma^*|\varsigma)\pi(S^*|\varsigma^*, \Lambda, \breve{\Phi}, \Psi)} \times \frac{\pi(\Lambda|S^*, \Psi)\pi(S^*|\varsigma^*, \breve{\Phi})\pi(\varsigma^*)}{\pi(\Lambda|S, \Psi)\pi(S|\varsigma, \breve{\Phi})\pi(\varsigma)} \\ &= \frac{q_1(\varsigma|\varsigma^*)\pi(S|\varsigma, \Lambda, \breve{\Phi}, \Psi)}{q_1(\varsigma^*|\varsigma)\pi(S^*|\varsigma^*, \Lambda, \breve{\Phi}, \Psi)} \times \frac{\pi(S^*|\varsigma^*, \Lambda, \breve{\Phi}, \Psi)\pi(\Lambda|\varsigma^*, \breve{\Phi}, \Psi)\pi(\varsigma^*)}{\pi(S|\varsigma, \Lambda, \breve{\Phi}, \Psi)\pi(\Lambda|\varsigma, \breve{\Phi}, \Psi)\pi(\varsigma)} \\ &= \frac{q_1(\varsigma|\varsigma^*)\pi(\Lambda|\varsigma^*, \breve{\Phi}, \Psi)\pi(\varsigma^*)}{q_1(\varsigma^*|\varsigma)\pi(\Lambda|\varsigma, \breve{\Phi}, \Psi)\pi(\varsigma)} \end{aligned}$$

where $\pi(\Lambda|\varsigma, \breve{\Phi}, \Psi)$ is the density of a matrix-$t$ random variable, $\Lambda|\varsigma, \breve{\Phi}, \Psi \sim \mathrm{t}_{p,k}(\varsigma, 0, \breve{\Phi}, \Psi)$, given by

$$p(\Lambda) = \frac{\Gamma_k\left\{(\varsigma + k + p - 1)/2\right\}}{\pi^{pk/2}\Gamma_k\left\{(\varsigma + k - 1)/2\right\}|\Psi|^{p/2}|\breve{\Phi}|^{k/2}} \det\left(I_p + \breve{\Phi}^{-1}\Lambda\Psi^{-1}\Lambda^{\mathrm{T}}\right)^{-(\varsigma+k+p-1)/2}.$$

Here $\Gamma_k(\cdot)$ denotes the multivariate gamma function, which can be expressed as $\Gamma_k(x) = \pi^{k(k-1)/4}\prod_{i=1}^{k}\Gamma\{x - \frac{1}{2}(i-1)\}$ if $\mathrm{Re}(x) > (k-1)/2$. We note that $A$ does not depend on $S^*$ and so $S$ need only be sampled if the proposed value of $\varsigma$ is accepted.

#### S4.1.2 Adaptive Gibbs sampler

Denote by $x^{[i]}$ the value of the unknown $x$ on iteration $i$ of the Gibbs sampler and suppose that adaptation is allowed after $\bar{i}$ iterations. Recall that we define the number of effective factors on iteration $i$ as $k^{*[i]} = H - m^{[i]}$ where $m^{[i]}$ is the number of columns of loadings that do not contribute appreciably to $\Omega^{[i]}$ according to a truncation criterion.

Iteration $i$ of the adaptive Gibbs sampler begins with a sweep through all the steps of the non-adaptive algorithm above. Then if $i \geq \bar{i}$, sample $u \sim \mathrm{U}(0, 1)$ and if $u < p(i)$ where $p(i) = \exp(\alpha_0 + \alpha_1 i)$, an adaptation step is carried out:

7. Compare $k^{*[i]}$ to $H$:
   (a) If $k^{*[i]} < H$, $H$ is reduced to $k^{*[i]}$ and any inactive factors are deleted along with the corresponding columns of $\Lambda$ and components of $\boldsymbol{\varrho}$ and $\Psi$ from the multiplicative gamma process prior.
   (b) If $k^{*[i]} = H$ and $H < \lceil\varphi(p)\rceil - 1$, an extra factor, component of $\boldsymbol{\varrho}$ and column of factor loadings are sampled from their priors. That is, we sample $\eta_{i,H+1} \sim \mathrm{N}(0, 1)$ $(i = 1, \ldots, n)$ and $\varrho_{H+1} \sim \mathrm{Gam}(a_1, 1)$ if $H = 0$ or $\varrho_{H+1} \sim \mathrm{Gam}(a_2, 1)$ otherwise. We then compute $\psi_{H+1} = 1/\varrho_{H+1}$ if $H = 0$ or $\psi_{H+1} = \psi_H/\varrho_{H+1}$ otherwise, and sample $\boldsymbol{\lambda}_{(1),H+1} \sim \mathrm{N}_p(\mathbf{0}, \psi_{H+1}\Phi)$. Finally, we increase $H$ by 1.

### S4.2 Gibbs samplers for dynamic factor models

#### S4.2.1 Gibbs sampler with fixed level of truncation

Consider the stationary dynamic factor model presented through equations (9) and (10) of the main manuscript and recall that $G_i = \mathrm{Cov}(\boldsymbol{\eta}_t, \boldsymbol{\eta}_{t+i})$ is the $i$th autocovariance of $\boldsymbol{\eta}_t$. The joint distribution of the factors can be expressed as

$$\begin{aligned} \pi(\boldsymbol{\eta}_{(1-m):n}|\Gamma_1, \ldots, \Gamma_m, \Pi) &= \pi(\boldsymbol{\eta}_{(1-m):0}|\Gamma_1, \ldots, \Gamma_m, \Pi) \\ &\quad \times \prod_{t=m+1}^{n} \pi(\boldsymbol{\eta}_t|\boldsymbol{\eta}_{(t-p):(t-1)}, \Gamma_1, \ldots, \Gamma_m, \Pi) \end{aligned} \tag{S15}$$

in which $\boldsymbol{\eta}_t|\boldsymbol{\eta}_{(t-m):(t-1)}, \Gamma_1, \ldots, \Gamma_m, \Pi \sim \mathrm{N}_k\left(\sum_{i=1}^{m}\Gamma_i\boldsymbol{\eta}_{t-i}\,, \Pi\right)$ and the initial distribution is $(\boldsymbol{\eta}_{1-m}^{\mathrm{T}}, \ldots, \boldsymbol{\eta}_0^{\mathrm{T}})^{\mathrm{T}}|\Gamma_1, \ldots, \Gamma_m, \Pi \sim \mathrm{N}_{km}(\mathbf{0}, G)$ where $G$ is a positive definite block Toeplitz

matrix with $G_{j-i}$ as the block in rows $\{k(i-1)+1\}$ to $ki$ and columns $\{k(j-1)+1\}$ to $kj$ $(i,j=1,\dots,m)$ and $G_{-k}=G_k^{\mathrm{T}}$ $(k=1,\dots,m-1)$. For the purposes of evaluating (S15), the stationary variance $G_0$ is fixed at $I_k$ and the autocovariances $G_1,\dots,G_{m-1}$, along with the innovation variance $\mathit{\Pi}$, are available as by-products of the reverse mapping from the unconstrained parameters $(A_1,\dots,A_m)$ to $(\mathit{\Gamma}_1,\dots,\mathit{\Gamma}_m)$; see the Appendix in Heaps (2022) for full details. The original parameters $(\mathit{\Gamma}_1,\dots,\mathit{\Gamma}_m,\mathit{\Pi})$ are therefore a complicated function of the unconstrained parameters $A_1,\dots,A_m$ and so the full conditional density of any particular $A_j$ can be written as

$$\pi(A_j|A_{-j},\boldsymbol{\eta}_{(1-m):n})\propto\pi(A_j)\pi(\boldsymbol{\eta}_{(1-m):n}|A_1,\dots,A_m), \tag{S16}$$

in which $A_{-j}$ denotes the collection $(A_1,\dots,A_m)$ with $A_j$ removed and $A_j\sim \mathrm{N}_{k,k}(\mathbf{0},I_k,I_k)$.

In order to extend the non-adaptive algorithm in the previous section to the dynamic case, we replace step 1 with

1. Sample $\boldsymbol{\eta}_{1-m},\dots,\boldsymbol{\eta}_n$ from their full conditional distribution as a single block using a forward-filtering backward-sampling algorithm (Carter and Kohn, 1994; Frühwirth-Schnatter, 1994).

We also add the following step between steps 2 and 3

2.5. For $j=1,\dots,m$ update $\mathrm{vec}(A_j)$ from its full conditional density (S16) using a Metropolis-adjusted Langevin (MALA) proposal

$$\mathrm{vec}(A_j^*)|\mathrm{vec}(A_j)\sim \mathrm{N}_{H^2}\left\{\mathrm{vec}(A_j)+\frac{s^2}{2}\bigtriangledown\log\pi(A_j|A_{-j},\boldsymbol{\eta}_{(1-m):n})\,,\,s^2 I_{H^2}\right\}$$

in which $\bigtriangledown\log\pi(A_j|A_{-j},\boldsymbol{\eta}_{(1-m):n})=\partial\log\pi(A_j|A_{-j},\boldsymbol{\eta}_{(1-m):n})/\partial\{\mathrm{vec}(A_j)\}^{\mathrm{T}}$ is the gradient of the logarithm of the full conditional density for $A_j$ and $s^2$ is a tuning variance.

If the acceptance rate is too small for reasonably sized $s$, we can divide each $A_j$ into blocks of length $b$ and use the approach above to update them one-at-a-time.

When the order of the vector autoregression in the state equation is $m=1$, $\bigtriangledown\log\pi(A_j|A_{-j},\boldsymbol{\eta}_{(1-m):n})$ can be calculated analytically; full details are given at the end of Section S4.2. When $m>1$, the gradients can be evaluated with automatic differentiation. Alternatively, the MALA steps can be replaced with Gaussian random walks.

### S4.2.2 Adaptive Gibbs sampler

As in the static case, the adaptive Gibbs sampler for a dynamic model begins with a sweep through all the steps of the non-adaptive scheme. In the adaptation step, an extra complication arises when the truncation point $H$ is increased by 1. Ideally, we would add a row and column to the parameters of the state equation, $\mathit{\Gamma}_1,\dots,\mathit{\Gamma}_m$, by sampling from their prior, conditional on the submatrices that already occupy the first $H$ rows and columns. However, in order to enforce stationarity, we work with a reparameterization of the vector autoregressive model for the factors. Priors are placed on the unconstrained parameters $A_1,\dots,A_m$ on which the parameters in the original model, $\mathit{\Gamma}_1,\dots,\mathit{\Gamma}_m,\mathit{\Pi}$, depend. Due to the recursive nature of the mapping between the original parameters and the intermediate partial autocorrelation parameterization $P_1,\dots,P_m$, the Jacobian of the transformation is not available in closed form and so neither is the prior for the original parameters over the stationary region. We cannot, therefore, simply sample extra rows and columns of the $\mathit{\Gamma}_i$ from their prior.

As an alternative, we propose basing the adaptation on the parsimonious assumption that the new factor does not interact with the existing factors at lags $1,\dots,m$ and interacts minimally with itself. This requires filling the first $H$ elements in row and column $H+1$ of

the adapted matrices $\mathit{\Gamma}_1, \dots, \mathit{\Gamma}_m$ with zeros. Equivalently, we can fill the first $H$ elements in row and column $H+1$ of the adapted partial autocorrelation matrices $P_1, \dots, P_m$ with zeros. The partial autocorrelation matrices lie in the space of square matrices whose singular values are all less than one. We can therefore guarantee a new parameter set that lies in the stationary region whilst adhering to our adaptation assumptions by simulating the $(H+1, H+1)$ element in the adapted $P_i$ by sampling uniformly on $(0, r_{i,\min})$ where $r_{i,\min}$ is the smallest singular value of $P_{i,1:H,1:H}$. We can then compute the corresponding value for $\mathit{\Pi}$ using step 2 of the reverse mapping in the Appendix of Heaps (2022).

Altogether, the adaptation step of the Gibbs sampler for a dynamic model replaces step 7 in the static case with the following:

7. Compare $k^{*[i]}$ to $H$:

   (a) If $k^{*[i]} < H$, $H$ is reduced to $k^{*[i]}$ and any inactive factors are deleted along with the corresponding columns of $\mathit{\Lambda}$, columns and rows of $(\mathit{\Gamma}_1, \dots, \mathit{\Gamma}_m, \mathit{\Pi})$, and components of $\boldsymbol{\varrho}$ and $\mathit{\Psi}$ from the multiplicative gamma process prior. We then recompute $(A_1, \dots, A_m)$.

   (b) If $k^{*[i]} = H$ and $H < \lceil \varphi(p) \rceil - 1$, an extra component of $\boldsymbol{\varrho}$ and column of factor loadings are sampled from their priors. That is, we sample $\varrho_{H+1} \sim \mathrm{Gam}(a_1, 1)$ if $H = 0$ or $\varrho_{H+1} \sim \mathrm{Gam}(a_2, 1)$ otherwise. We then compute $\psi_{H+1} = 1/\varrho_{H+1}$ if $H = 0$ or $\psi_{H+1} = \psi_H/\varrho_{H+1}$ otherwise, and sample $\boldsymbol{\lambda}_{(1),H+1} \sim \mathrm{N}_p(\mathbf{0}, \psi_{H+1}\mathit{\Phi})$. For $i = 1, \dots, m$, we set $p_{i,H+1,j} = p_{i,j,H+1} = 0$ for $j = 1, \dots, H$ and sample $p_{i,H+1,H+1} \sim \mathrm{U}(0, r_{i,\min})$. We then recompute $(A_1, \dots, A_m)$ and $\mathit{\Pi}$. We additionally compute $(\mathit{\Gamma}_1, \dots, \mathit{\Gamma}_m)$ and $G$ so that we can sample an extra factor $(\eta_{1-m,H+1}, \dots, \eta_{n,H+1})^{\mathrm{T}}$ from the implied univariate autoregressive model of order $m$. That is, we sample $(\eta_{1-m,H+1}, \dots, \eta_{0,H+1})^{\mathrm{T}} \sim \mathrm{N}_m(\mathbf{0}, G^*)$ and then $\eta_{t,H+1} \sim \mathrm{N}(\sum_{i=1}^m \gamma_{i,H+1,H+1}\eta_{t-i,H+1}, \pi_{H+1,H+1})$ for $t = 1, \dots, n$, where $G^*$ comprises the submatrix of $G$ made up of rows and columns $(H+1, 2H+2, \dots, mH+m)$. Finally, we increase $H$ by 1.

### S4.2.3 Gradient of the logarithm of the full conditional density when $m = 1$

In the special case when $m = 1$, there are closed form expressions for the lag-1 autoregressive coefficient matrix $\mathit{\Gamma}_1$ and the innovation variance $\mathit{\Pi}$ in terms of the transformed partial autocorrelation matrix $A_1$. Dropping the 1-subscript for brevity, we can write $\mathit{\Gamma} = (I_k + AA^{\mathrm{T}})^{-1/2}A$ and $\mathit{\Pi} = (I_k + AA^{\mathrm{T}})^{-1}$. This allows the joint density of the factors (S15), and hence the logarithm of the full conditional density for $A$, to be written as a closed form function of $A$. Up to an additive constant of proportionality, we have

$$\begin{aligned}\log \pi(A|\boldsymbol{\eta}_{0:n}) &= \frac{n}{2}\log|I_k + AA^{\mathrm{T}}| - \frac{1}{2}\mathrm{tr}(AA^{\mathrm{T}}) \\ &\quad - \frac{1}{2}\sum_{t=1}^{n}\left\{\boldsymbol{\eta}_t^{\mathrm{T}}AA^{\mathrm{T}}\boldsymbol{\eta}_t - 2\boldsymbol{\eta}_t^{\mathrm{T}}(I_k + AA^{\mathrm{T}})^{1/2}A\boldsymbol{\eta}_{t-1} + \boldsymbol{\eta}_{t-1}^{\mathrm{T}}AA^{\mathrm{T}}\boldsymbol{\eta}_{t-1}\right\}.\end{aligned} \tag{S17}$$

whose gradient can be derived analytically.

**Theorem 2.** *The gradient of the logarithm of the full conditional density in* (S17) *is given*

*by*

$$\frac{\partial \log \pi(A|\boldsymbol{\eta}_{0:n})}{\partial\{(\mathrm{vec}(A)\}^{\mathrm{T}}} = \frac{n}{2}\mathrm{vec}\left\{(I_k + AA^{\mathrm{T}})^{-1}\right\}^{\mathrm{T}}(I_{k^2} + I_{(k,k)})(A \otimes I_k) - \mathrm{vec}(A)^{\mathrm{T}}$$
$$- \frac{1}{2}\sum_{t=1}^{n}\Bigg((\eta_t^{\mathrm{T}} \otimes \eta_t^{\mathrm{T}})(I_{k^2} + I_{(k,k)})(A \otimes I_k) + (\eta_{t-1}^{\mathrm{T}} \otimes \eta_{t-1}^{\mathrm{T}})(I_{k^2} + I_{(k,k)})(I_k \otimes A^{\mathrm{T}})$$
$$- 2(\eta_{t-1}^{\mathrm{T}} \otimes \eta_t^{\mathrm{T}})\Big[(A \otimes I_k)^{\mathrm{T}}\{(I_k + AA^{\mathrm{T}})^{1/2} \oplus (I_k + AA^{\mathrm{T}})^{1/2}\}^{-1}(I_{k^2} + I_{(k,k)})(A \otimes I_k)$$
$$+ I_k \otimes (I_k + AA^{\mathrm{T}})^{1/2}\Big]\Bigg).$$

*Proof.* In order to compute the gradient of (S17) we make extensive use of the results from Chapter 17 of Seber (2008), as detailed below. From Result 17.30(g),

$$\frac{\partial}{\partial \mathrm{vec}(A)^{\mathrm{T}}}\mathrm{vec}(AA^{\mathrm{T}}) = (I_{k^2} + I_{(k,k)})(A \otimes I_k)$$

and so, using Result 17.33(a) yields

$$\frac{\partial}{\partial \mathrm{vec}(A)^{\mathrm{T}}}(\eta_t^{\mathrm{T}} AA^{\mathrm{T}}\eta_t) = (\eta_t^{\mathrm{T}} \otimes \eta_t^{\mathrm{T}})\frac{\partial}{\partial \mathrm{vec}(A)^{\mathrm{T}}}\mathrm{vec}(AA^{\mathrm{T}})$$
$$= (\eta_t^{\mathrm{T}} \otimes \eta_t^{\mathrm{T}})(I_{k^2} + I_{(k,k)})(A \otimes I_k) \tag{S18}$$

in which $I_{(k,k)}$ denotes a vec-permutation (or commutation) matrix, that is, the $k^2 \times k^2$ permutation matrix such that $\mathrm{vec}(A) = I_{(k,k)}\mathrm{vec}(A^{\mathrm{T}})$.

Similarly, using Result 17.30(f)

$$\frac{\partial}{\partial \mathrm{vec}(A)^{\mathrm{T}}}\mathrm{vec}(A^{\mathrm{T}}A) = (I_{k^2} + I_{(k,k)})(I_k \otimes A^{\mathrm{T}})$$

and so, using Result 17.33(a) again yields

$$\frac{\partial}{\partial \mathrm{vec}(A)^{\mathrm{T}}}\left(\eta_{t-1}^{\mathrm{T}} A^{\mathrm{T}}A\eta_{t-1}\right) = (\eta_{t-1}^{\mathrm{T}} \otimes \eta_{t-1}^{\mathrm{T}})\frac{\partial}{\partial \mathrm{vec}(A)^{\mathrm{T}}}\mathrm{vec}(A^{\mathrm{T}}A)$$
$$= (\eta_{t-1}^{\mathrm{T}} \otimes \eta_{t-1}^{\mathrm{T}})(I_{k^2} + I_{(k,k)})(I_k \otimes A^{\mathrm{T}}). \tag{S19}$$

From Results 17.30(h) and 17.30(a), we have

$$\frac{\partial}{\partial \mathrm{vec}(A)^{\mathrm{T}}}\mathrm{vec}\left\{(I_k + AA^{\mathrm{T}})^{1/2}A\right\}$$
$$= (A \otimes I_k)^{\mathrm{T}}\frac{\partial}{\partial \mathrm{vec}(A)^{\mathrm{T}}}\mathrm{vec}\left\{(I_k + AA^{\mathrm{T}})^{1/2}\right\} + \left\{I_k \otimes (I_k + AA^{\mathrm{T}})^{1/2}\right\}\frac{\partial \mathrm{vec}A}{\partial \mathrm{vec}(A)^{\mathrm{T}}}$$
$$= (A \otimes I_k)^{\mathrm{T}}\frac{\partial}{\partial \mathrm{vec}(A)^{\mathrm{T}}}\mathrm{vec}\left\{(I_k + AA^{\mathrm{T}})^{1/2}\right\} + I_k \otimes (I_k + AA^{\mathrm{T}})^{1/2}. \tag{S20}$$

Now, using Result 17.31, with $F(A) = Z\{Y(A)\}$ where $Z(V) = V^{1/2}$ and $Y(A) = I_k + AA^{\mathrm{T}}$, we have

$$\frac{\partial \mathrm{vec}(F)}{\partial \mathrm{vec}(A)^{\mathrm{T}}} = \left.\frac{\partial \mathrm{vec}\{Z(V)\}}{\partial\{\mathrm{vec}(V)\}^{\mathrm{T}}}\right|_{V=Y(A)}\frac{\partial \mathrm{vec}\{Y(A)\}}{\partial \mathrm{vec}(A)^{\mathrm{T}}}. \tag{S21}$$

Using Result 17.30(g) again we have

$$\frac{\partial \mathrm{vec}\{Y(A)\}}{\partial \mathrm{vec}(A)^{\mathrm{T}}} = (I_{k^2} + I_{(k,k)})(A \otimes I_k). \tag{S22}$$

In order to compute $\partial \text{vec}\{Z(V)\}/\partial\{\text{vec}(V)\}^{\mathrm{T}} = \partial \text{vec}(V^{1/2})/\partial\{\text{vec}(V)\}^{\mathrm{T}}$ we first note that

$$V^{1/2}V^{1/2} = V.$$

Taking the differential of each side and noting that $V^{1/2}$ is a symmetric matrix yields

$$V^{1/2}dV^{1/2} + (dV^{1/2})V^{1/2} = dV.$$

This can be regarded as a Sylvester equation in $dV^{1/2}$ which can be rewritten as

$$(I_k \otimes V^{1/2} + V^{1/2} \otimes I_k)\text{vec}(dV^{1/2}) = (V^{1/2} \oplus V^{1/2})\text{vec}(dV^{1/2}) = \text{vec}(dV)$$

in which $\oplus$ is the Kronecker sum operator. Using Result 17.56(e) we can write this as

$$(V^{1/2} \oplus V^{1/2})d\text{vec}(V^{1/2}) = d\text{vec}(V).$$

Since $V^{1/2}$ is positive definite, $(V^{1/2} \oplus V^{1/2})$ will also be positive definite and so

$$d\text{vec}(V^{1/2}) = (V^{1/2} \oplus V^{1/2})^{-1}d\text{vec}(V).$$

We can then use Result 17.58 to obtain

$$\frac{\partial \text{vec}(V^{1/2})}{\partial \text{vec}(V)^{\mathrm{T}}} = (V^{1/2} \oplus V^{1/2})^{-1}. \tag{S23}$$

Taking (S22) and (S23) in (S21) gives

$$\frac{\partial}{\partial \text{vec}(A)^{\mathrm{T}}}\text{vec}\left\{(I_k + AA^{\mathrm{T}})^{1/2}\right\} = \{(I_k + AA^{\mathrm{T}})^{1/2} \oplus (I_k + AA^{\mathrm{T}})^{1/2}\}^{-1}(I_{k^2} + I_{(k,k)})(A \otimes I_k)$$

which can be substituted into (S20) to obtain

$$\begin{aligned}\frac{\partial}{\partial \text{vec}(A)^{\mathrm{T}}}\text{vec}\left\{(I_k + AA^{\mathrm{T}})^{1/2}A\right\} &= (A \otimes I_k)^{\mathrm{T}}\{(I_k + AA^{\mathrm{T}})^{1/2} \oplus (I_k + AA^{\mathrm{T}})^{1/2}\}^{-1} \\ &\quad \times (I_{k^2} + I_{(k,k)})(A \otimes I_k) + I_k \otimes (I_k + AA^{\mathrm{T}})^{1/2}.\end{aligned}$$

Finally, from Result 17.33(a) we have

$$\begin{aligned}&\frac{\partial}{\partial \text{vec}(A)^{\mathrm{T}}}\left\{\eta_t^{\mathrm{T}}(I_k + AA^{\mathrm{T}})^{1/2}A\eta_{t-1}\right\} \\ &\quad = (\eta_{t-1}^{\mathrm{T}} \otimes \eta_t^{\mathrm{T}})\frac{\partial}{\partial \text{vec}(A)^{\mathrm{T}}}\text{vec}\left\{(I_k + AA^{\mathrm{T}})^{1/2}A\right\} \\ &\quad = (\eta_{t-1}^{\mathrm{T}} \otimes \eta_t^{\mathrm{T}})\Big[(A \otimes I_k)^{\mathrm{T}}\{(I_k + AA^{\mathrm{T}})^{1/2} \oplus (I_k + AA^{\mathrm{T}})^{1/2}\}^{-1}(I_{k^2} + I_{(k,k)})(A \otimes I_k) \\ &\qquad + I_k \otimes (I_k + AA^{\mathrm{T}})^{1/2}\Big].\end{aligned} \tag{S24}$$

Denoting by $\text{adj}(X)$ the adjoint of a square matrix $X$, using Result 17.26(c) with Result 17.30(g) gives

$$\begin{aligned}\frac{\partial}{\partial \text{vec}(A)^{\mathrm{T}}}|I_k + AA^{\mathrm{T}}| &= \text{vec}\left[\{\text{adj}(I_k + AA^{\mathrm{T}})\}^{\mathrm{T}}\right]^{\mathrm{T}}\frac{\partial}{\partial \text{vec}(A)^{\mathrm{T}}}\text{vec}(I_k + AA^{\mathrm{T}}) \\ &= \text{vec}\left\{|I_k + AA^{\mathrm{T}}|(I_k + AA^{\mathrm{T}})^{-1}\right\}^{\mathrm{T}}(I_{k^2} + I_{(k,k)})(A \otimes I_k)\end{aligned}$$

and then applying the Chain Rule (Result 17.21) gives

$$\begin{aligned}&\frac{\partial}{\partial \text{vec}(A)^{\mathrm{T}}}\log|I_k + AA^{\mathrm{T}}| \\ &\quad = \frac{1}{|I_k + AA^{\mathrm{T}}|}\text{vec}\left\{|I_k + AA^{\mathrm{T}}|(I_k + AA^{\mathrm{T}})^{-1}\right\}^{\mathrm{T}}(I_{k^2} + I_{(k,k)})(A \otimes I_k) \\ &\quad = \text{vec}\left\{(I_k + AA^{\mathrm{T}})^{-1}\right\}^{\mathrm{T}}(I_{k^2} + I_{(k,k)})(A \otimes I_k).\end{aligned} \tag{S25}$$

Finally, for the contribution from the prior, we can compute

$$\frac{\partial}{\partial \text{vec}(A)} \left\{ -\frac{1}{2} \text{tr}(AA^{\text{T}}) \right\} = -\text{vec}(A)$$

which follows from Result 17.23. Therefore

$$\frac{\partial}{\partial \text{vec}(A)^{\text{T}}} \left\{ -\frac{1}{2} \text{tr}(AA^{\text{T}}) \right\} = -\text{vec}(A)^{\text{T}}. \tag{S26}$$

Combining (S18), (S19), (S24), (S25) and (S26) gives the required gradient. □

### S4.3 Diagnostic checking

Recall that we denote by $\Lambda$ a factor loadings matrix that is unconstrained and by $\tilde{\Lambda}$ one that is constrained by the PLT condition. The main manuscript provides formulae for computing identified parameters from their counterparts in the parameter-expanded factor models; see Sections 3.1 and 4.4 for static and dynamic models, respectively. The MCMC samplers described in this work generate draws from the posteriors of unknowns in the parameter-expanded models. However, the ability to post-process these draws to obtain samples of identifiable parameters is crucial for diagnostic checking. To illustrate, Figure S1 shows some graphical diagnostics from the analysis of the Finnish bird data in Section 6.1 of the main manuscript. In these plots the four different colours correspond to the output under four chains: two adaptive Gibbs chains and two Hamiltonian Monte Carlo chains implemented using Stan. The first two columns show diagnostics for two selected parameters from the parameter-expanded factor loadings matrix, namely $\lambda_{8,1}$ and $\lambda_{27,1}$. The second two columns show diagnostics for parameters in the corresponding positions of the identified factor loadings matrix, $\tilde{\lambda}_{8,1}$ and $\tilde{\lambda}_{27,1}$. The lack of identifiability of the parameter-expanded matrix is very clear. The two marginal posterior densities are multimodal with two major modes that are symmetric about zero. These arise because both the likelihood and prior are invariant to a flip of the sign of each column of the parameter-expanded factor loadings matrix. Some of the chains find and remain in one of the two modes, others occasionally jump between modes. In terms of the factor model, these modes are equivalent; indeed, we see no evidence of any lack of convergence or problems with mixing in the diagnostics for the identified parameters, and this was true for all other unknowns in $\tilde{\Lambda}$. However, it demonstrates the importance of basing diagnostic checks on samples of the identifiable parameters $\tilde{\Lambda}$ rather than the non-identifiable parameters $\Lambda$; using samples of $\Lambda$, one cannot distinguish confidently between artefacts of non-identifiability and genuine failed convergence of the sampler.

## S5 Further details on applications

### S5.1 Co-occurrence of Finnish birds

#### S5.1.1 Posterior summaries

The marginal correlation matrix is given by $S_\Omega^{-1} \Omega S_\Omega^{-1}$, where $S_\Omega = \text{diag}(\sqrt{\omega_{11}}, \dots, \sqrt{\omega_{pp}})$. Figure S2 shows the mean of the posterior for the marginal correlation matrix under the structured matrix-$t$ prior. The order of the 50 bird species is based on their phylogenetic tree, which is shown in the margins of the plot. There is clear structure in the matrix with several groups of species that share a recent common ancestor displaying strong positive correlations. This includes the species in the first ten rows, which correspond to birds from the Corvoidea superfamily and the Sylviidae family; the species in rows 19 to 30, which correspond largely to birds from the Musicapoidea superfamily; and the species in rows 42 to 47, which correspond mostly to birds from the Scolopacidae superfamily. It is also clear that

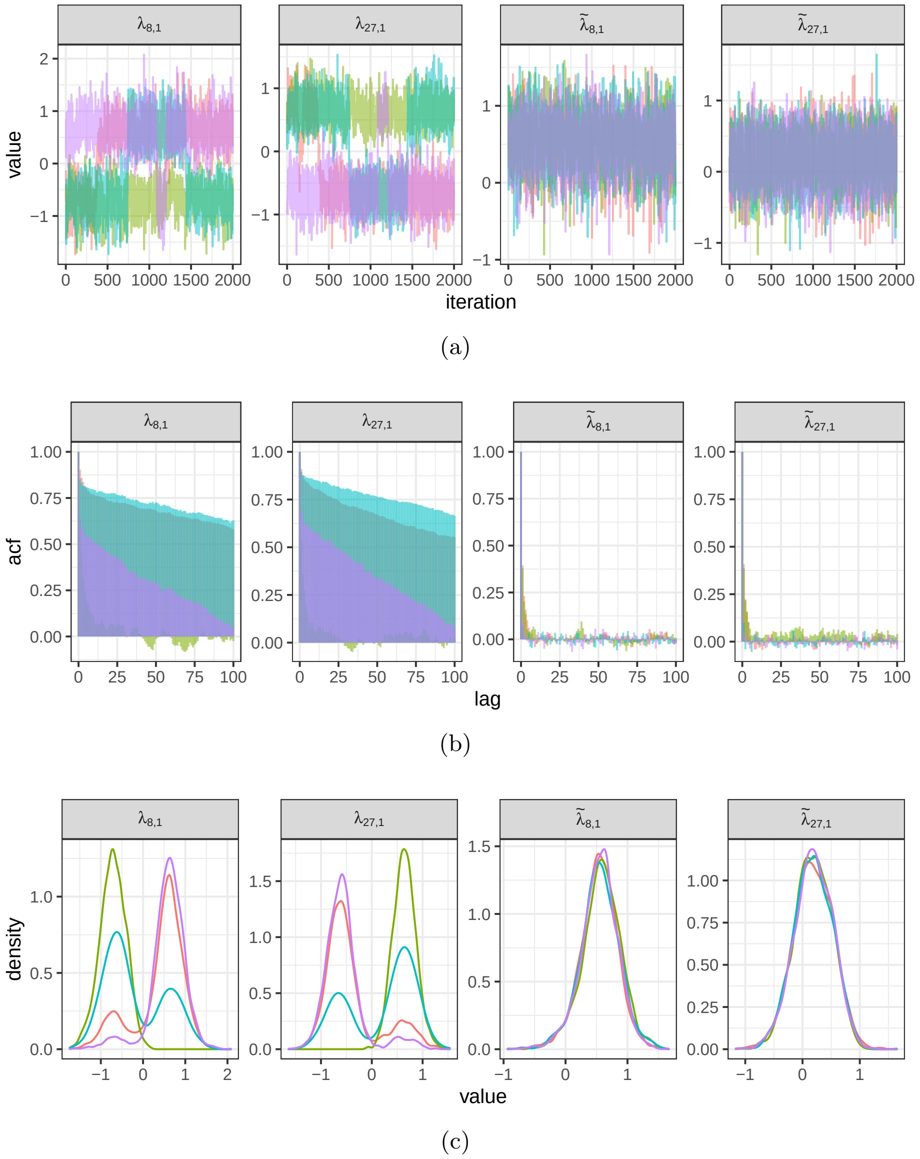


Figure S1: Graphical diagnostics for two parameters from the unconstrained factor loadings matrix ($\lambda_{8,1}$ and $\lambda_{27,1}$) and two parameters from the factor loadings matrix identified by the PLT constraint ($\tilde{\lambda}_{8,1}$ and $\tilde{\lambda}_{27,1}$): (a) trace plots, (b) autocorrelation plots and (c) marginal density plots. Different colours depict the output from two Gibbs chains (—, —) and two Hamiltonian Monte Carlo chains run using Stan (—, —).

most of the rows and columns predominated by near-zero correlations correspond to basal species, like *Columba palumbus* and *Grus grus*. Nevertheless, the structure of the matrix is clearly not dictated by evolutionary proximity alone. This message is reinforced by a plot of the corresponding correlation matrix from the model that fixes $\delta_{ij} = \psi\phi_{ij} = \psi \exp(-d_{ij})$, which is shown in Figure S3. Although this plot displays some of the same features as Figure S2, there are notable differences between them. For example, the restrictive model suggests there are strong relationships between the species in the Passeroidea superfamily, in rows 30 to 41, but this is not apparent under the more flexible factor model with structured matrix-$t$ prior. Interestingly, the corresponding plot in Figure S4 from the analysis under the structured increasing shrinkage process prior appears to be very sparse. At least in part, this can be attributed to shrinkage of $\varDelta$ towards its prior mean, which is a diagonal matrix.

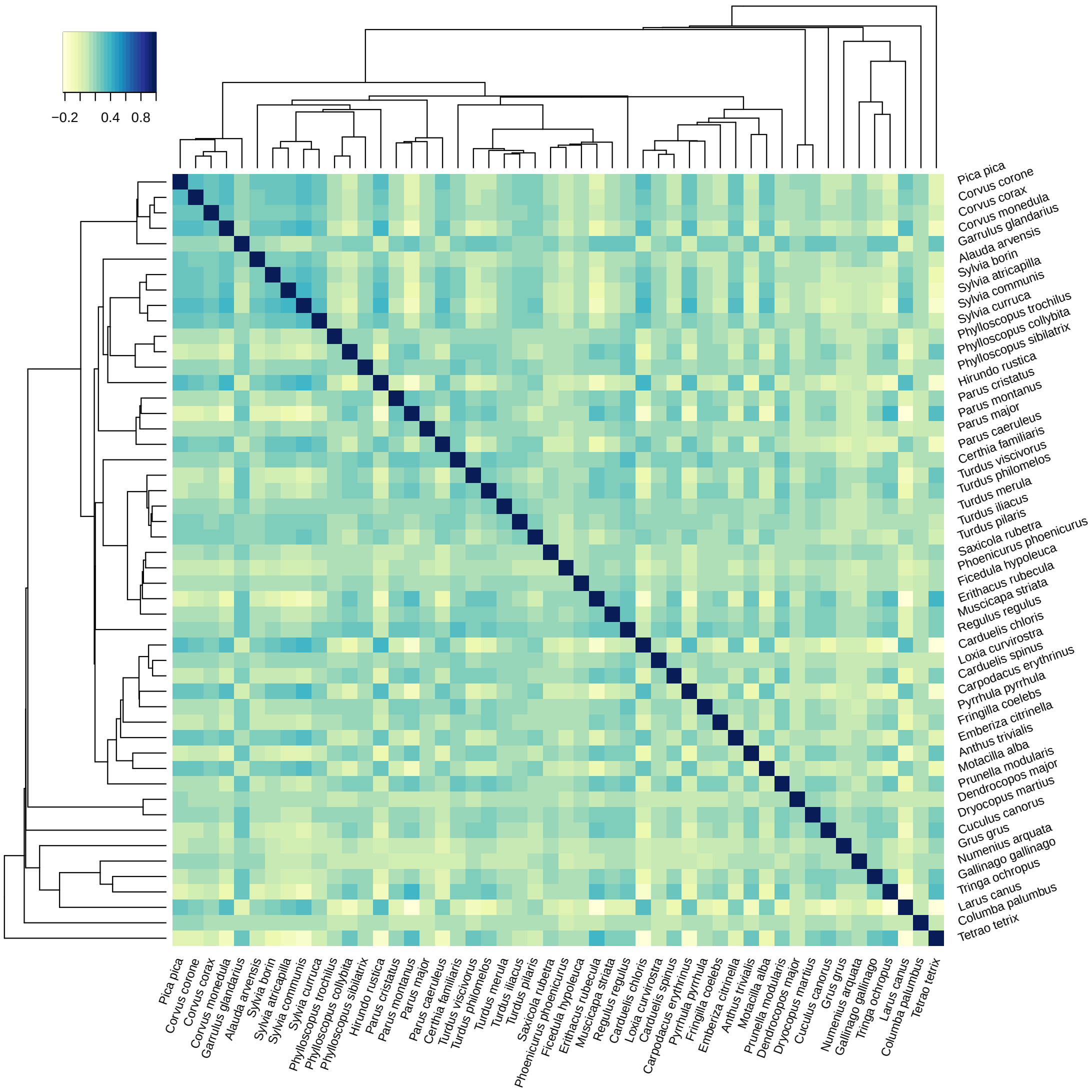


Figure S2: Mean of the posterior for the marginal correlation matrix under the structured matrix-$t$ prior. The species are ordered according to their phylogenetic tree which is visualized in the margins.

### S5.1.2 Pseudo marginal likelihood

Denote by $\boldsymbol{\theta}$ the set of all parameters in any of the three model-prior combinations discussed in the main manuscript. Recall that the $n \times p$ binary matrix of occurrences of birds is denoted by $Y$. Let $\boldsymbol{y}_i^{\mathrm{T}}$ represent the $i$th row of $Y$ and $Y_{-i}$ represent $Y$ with the $i$th row removed. The pseudo marginal likelihood can then be defined as

$$\mathrm{PML}(Y) = \prod_{i=1}^{n} p(\boldsymbol{y}_i | Y_{-i}) = \prod_{i=1}^{n} \int p(\boldsymbol{y}_i|\boldsymbol{\theta})\pi(\boldsymbol{\theta}|Y_{-i}) d\boldsymbol{\theta} \simeq \prod_{i=1}^{n} \int p(\boldsymbol{y}_i|\boldsymbol{\theta})\pi(\boldsymbol{\theta}|Y) d\boldsymbol{\theta},$$

in which the approximation on the third line allows $\mathrm{PML}(Y)$ to be approximated from the output of a single sample, $\boldsymbol{\theta}^{[1]}, \ldots, \boldsymbol{\theta}^{[B]}$, from the full posterior $\pi(\boldsymbol{\theta}|Y)$ through

$$\mathrm{PML}(Y) \simeq \prod_{i=1}^{n} \frac{1}{B} \sum_{b=1}^{B} p(\boldsymbol{y}_i|\boldsymbol{\theta}^{[b]}).$$

In practice, each of the terms $p(\boldsymbol{y}_i|\boldsymbol{\theta}^{[b]})$ is a multivariate normal probability which is approximated using the `pmvnorm` function from the `mvtnorm` package in R (Genz et al., 2021; Genz and Bretz, 2009).

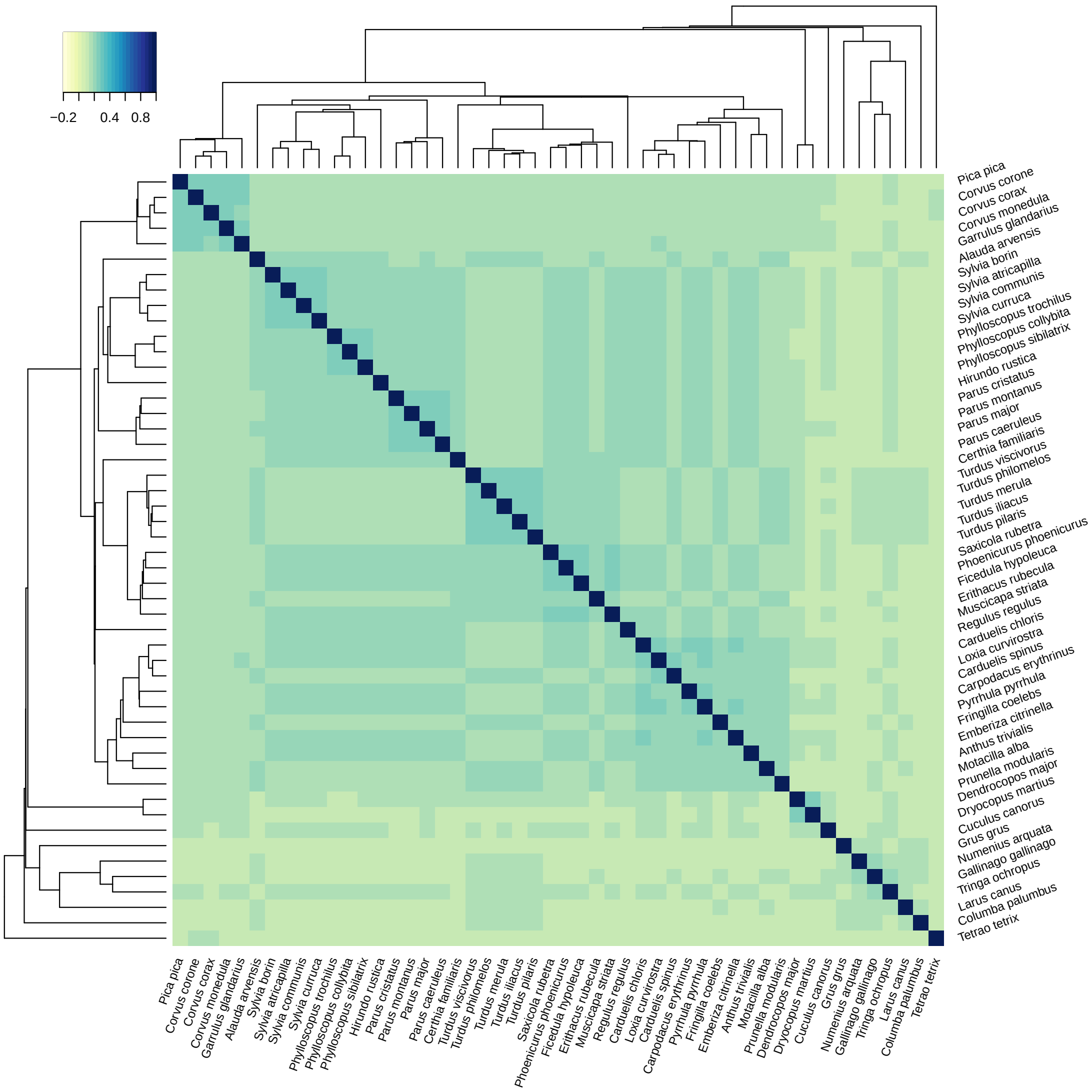


Figure S3: Mean of the posterior for the marginal correlation matrix under the parametric form model. The species are ordered according to their phylogenetic tree which is visualized in the margins.

### S5.1.3 Proper scoring rules

The Brier and logarithmic scores can readily be calculated using output from the MCMC sampler (Gschlößl and Czado, 2008). For species $j$ and a new sampling location $i$, the posterior predictive probability that $y_{ij}$ is equal to 1 can be calculated through

$$p_{ij} = \int \Pr(y_{ij} = 1|\boldsymbol{\theta})\pi(\boldsymbol{\theta}|Y) \simeq \frac{1}{B}\sum_{b=1}^{B} \Pr(y_{ij} = 1|\boldsymbol{\theta}^{[b]})$$

in which $\boldsymbol{\theta}^{[1]}, \ldots, \boldsymbol{\theta}^{[B]}$ are a sample from the posterior $\pi(\boldsymbol{\theta}|Y)$. In order to use all the observations as both test data and training data, we adopt a 4-fold cross-validation approach, randomly assigning the $n = 137$ observations into 4 folds. Denote by $f(k)$ the subset of $\{1, \ldots, n\}$ containing observations assigned to fold $k$ and by $Y_{-f(k)}$ the occurrence matrix with the rows in $f(k)$ removed. We can then calculate

$$p_{ij} \simeq \frac{1}{B}\sum_{b=1}^{B} \Pr(y_{ij} = 1|\boldsymbol{\theta}^{[b]}), \quad \boldsymbol{\theta}^{[b]} \sim \pi(\boldsymbol{\theta}|Y_{-f(k)}), \quad b = 1, \ldots, B$$

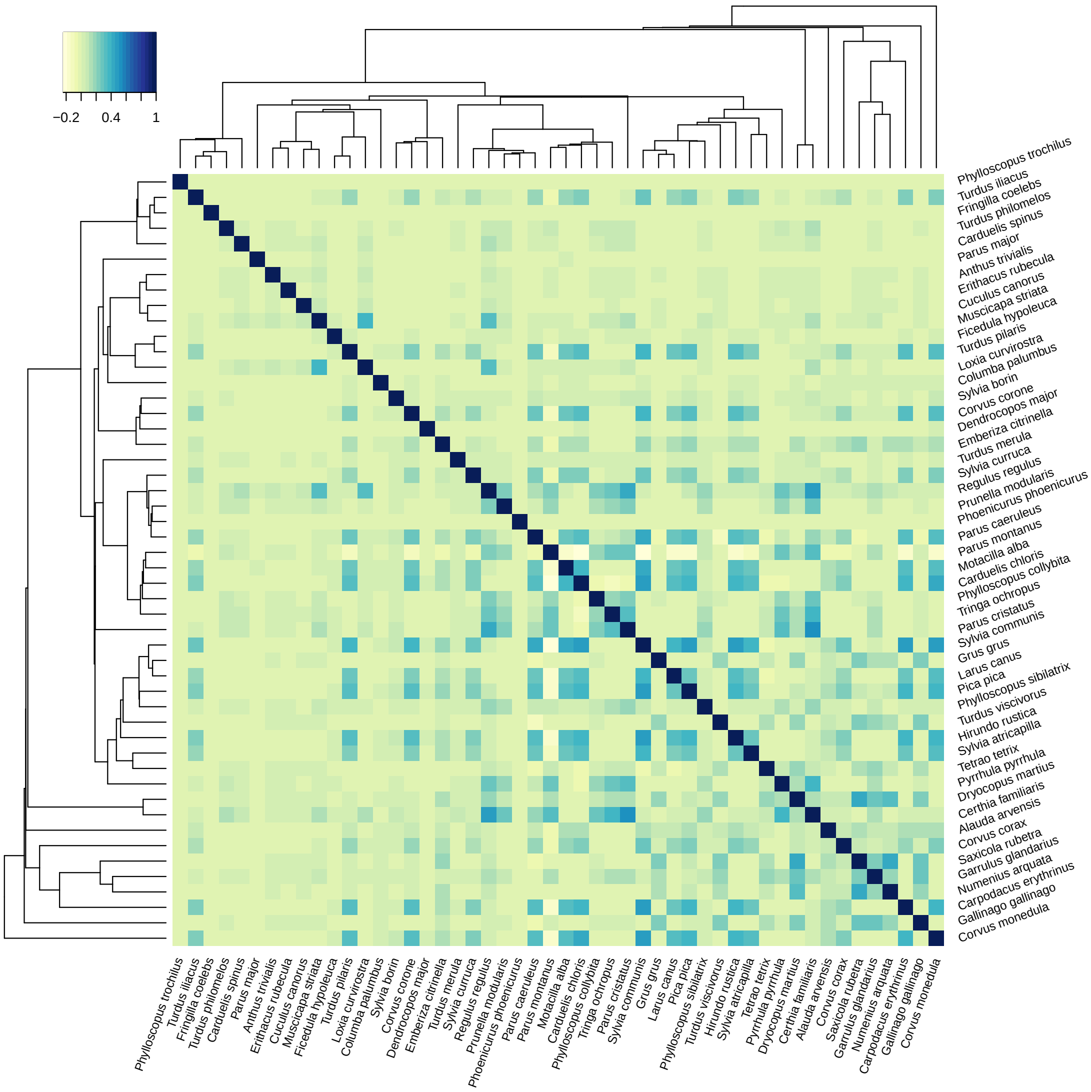


Figure S4: Mean of the posterior for the marginal correlation matrix under the structured increasing shrinkage process prior. The species are ordered according to their phylogenetic tree which is visualized in the margins.

for $i \in f(k)$, $j = 1, \ldots, p = 50$ and $k = 1, \ldots, 4$. The different model-prior combinations can then be compared based on the mean score

$$S = \frac{1}{np} \sum_{i=1}^{n} \sum_{j=1}^{p} S(p_{ij}, y_{ij}).$$

The Brier score is defined as

$$S(p_{ij}, y_{ij}) = -2(p_{ij} - y_{ij})^2$$

while the logarithmic score is defined as

$$S(p_{ij}, y_{ij}) = y_{ij} \log p_{ij} + (1 - y_{ij}) \log(1 - p_{ij}).$$

## S5.2 Hourly demand for natural gas

### S5.2.1 Model for the time-varying mean

Each term in the time-varying mean $\boldsymbol{\mu}_t = (\mu_{t1}, \ldots, \mu_{t,24})^{\mathrm{T}}$ can be written as

$$\mu_{ti} = \beta_{1i} + (\beta_{2i} + \beta_{3i}\tilde{w}_t)w_{t2} + \beta_{4i}w_{t4} + \chi_{ti} + \varpi_{ti}$$

where $\tilde{w}_t$ is the temperature for day $t$ and $w_{t2} = \tilde{w}_t - m_{d(t)}$ in which $m_{d(t)}$ is a smoothed annual average for the temperature on day $t$ where $d(t) \in \{1, 2, \ldots, 366\}$. We include both the mean-centered temperature, $w_{t2}$, and its interaction with the raw temperature, $w_{t3} = \tilde{w}_t w_{t2}$, to allow the effect of above or below average temperatures to differ according to absolute weather conditions. The variable $w_{t4}$ is an indicator that is equal to 1 if day $t$ is a public holiday and equal to zero otherwise.

The term $\chi_{ti}$ gives a day-of-the-week effect, whilst $\varpi_{ti}$ gives a seasonal or, day-of-the-year, effect. Both terms are composed using Fourier series with

$$\chi_{ti} = \sum_{k=1}^{3} \left\{ \beta_{4+2(k-1)+1,i} \cos\left(\frac{2\pi k t}{7}\right) + \beta_{4+2k,i} \sin\left(\frac{2\pi k t}{7}\right) \right\} \tag{S27}$$

and

$$\varpi_{ti} = \sum_{k=1}^{K} \left\{ \beta_{10+2(k-1)+1,i} \cos\left(\frac{2\pi k t}{365.25}\right) + \beta_{10+2k,i} \sin\left(\frac{2\pi k t}{365.25}\right) \right\}. \tag{S28}$$

The six unconstrained coefficients in (S27) provide fixed effects for each day of the week which, by construction, sum to zero. The advantages of this parameterization are that the six coefficients are unconstrained and by treating them as exchangeable *a priori*, we can induce a prior for the seven fixed effects which is symmetric with respect to the day of the week. The Fourier series for the seasonal term in (S28) is truncated at $K = 6$ harmonics based on analysis similar data that suggested the contribution of higher frequency harmonics was negligible (Heaps et al., 2020).

Row $i$ of the $c \times p$ matrix of regression coefficients $B = (\beta_{ij})$ characterizes the effect of the $i$th covariate on the demand for gas across the $p = 24$ hours of the day. In the prior we assume the coefficients on different rows are independent but allow borrowing of strength within each row by assigning a hierarchical prior. For row $i$, $i = 1, \ldots, c$, this takes the form

$$\beta_{ij} | \mu_{\beta,i}, \sigma^2_{\beta,i} \sim \mathrm{N}(\mu_{\beta,i}, \sigma^2_{\beta,i})$$

for $j = 1, \ldots, p$ in which $\mu_{\beta,i} \sim \mathrm{N}(0, 7)$ and $1/\sigma^2_{\beta,i} \sim \gamma(21, 60)$.

### S5.2.2 Posterior summaries

Let $\Upsilon = \Omega^{-1} = (\upsilon_{ij})$ denote the marginal precision matrix of the process and let $S_\Upsilon = \mathrm{diag}(\sqrt{\upsilon_{11}}, \ldots, \sqrt{\upsilon_{pp}})$. Figure S5 shows the posterior mean for the standardized precision matrix $S_\Upsilon^{-1} \Upsilon S_\Upsilon^{-1}$. It is clear that its structure is reasonably consistent with the tridiagonal Toeplitz matrix with corners on which the prior for $\Delta^{-1}$ is centered. However, there are some deviations, most notably another one or two bands of non-zero elements below the subdiagonal and above the supradiagonal. There is also some evidence of at least a partial band in the vicinity of $\upsilon_{i,i+12}$ for $i = 1, \ldots, 12$. This may be due to people switching their heating on twice per day, at around 7:00 in the morning and around 19:00 in the evening.

The observation equation of the identified model $\boldsymbol{y}_t = \boldsymbol{\mu}_t + \tilde{\Lambda} \tilde{\boldsymbol{\eta}}_t + \boldsymbol{\epsilon}_t$ suggests that we can interpret the columns of the identified factor loadings matrix $\tilde{\Lambda}$ as typical *gas-day-profiles*; on any particular day, $\boldsymbol{y}_t - \boldsymbol{\mu}_t$ is simply a noisy weighted sum of gas-day-profiles, and these weights evolve over time. Figure S6 shows the posterior mean for the identified factor loadings matrix $\tilde{\Lambda}$. It appears that many of the columns have a double-hump shape with smaller loadings towards the middle of the gas-day. This is also apparent in Figure S7 which shows a more complete summary of the marginal posterior densities for the loadings of the first three factors, $\tilde{\lambda}_{ii}, \ldots, \tilde{\lambda}_{24,i}$ for $i = 1, 2, 3$. Again, this may be due to people switching their heating on twice per day and is therefore consistent with conclusions drawn from the posterior mean of the marginal precision matrix

Figure 2 in the paper showed a plot of the 1– and 24-step ahead posterior predictive distributions for the first 5% of times in the hold-out period. Figure S8 shows an analogous

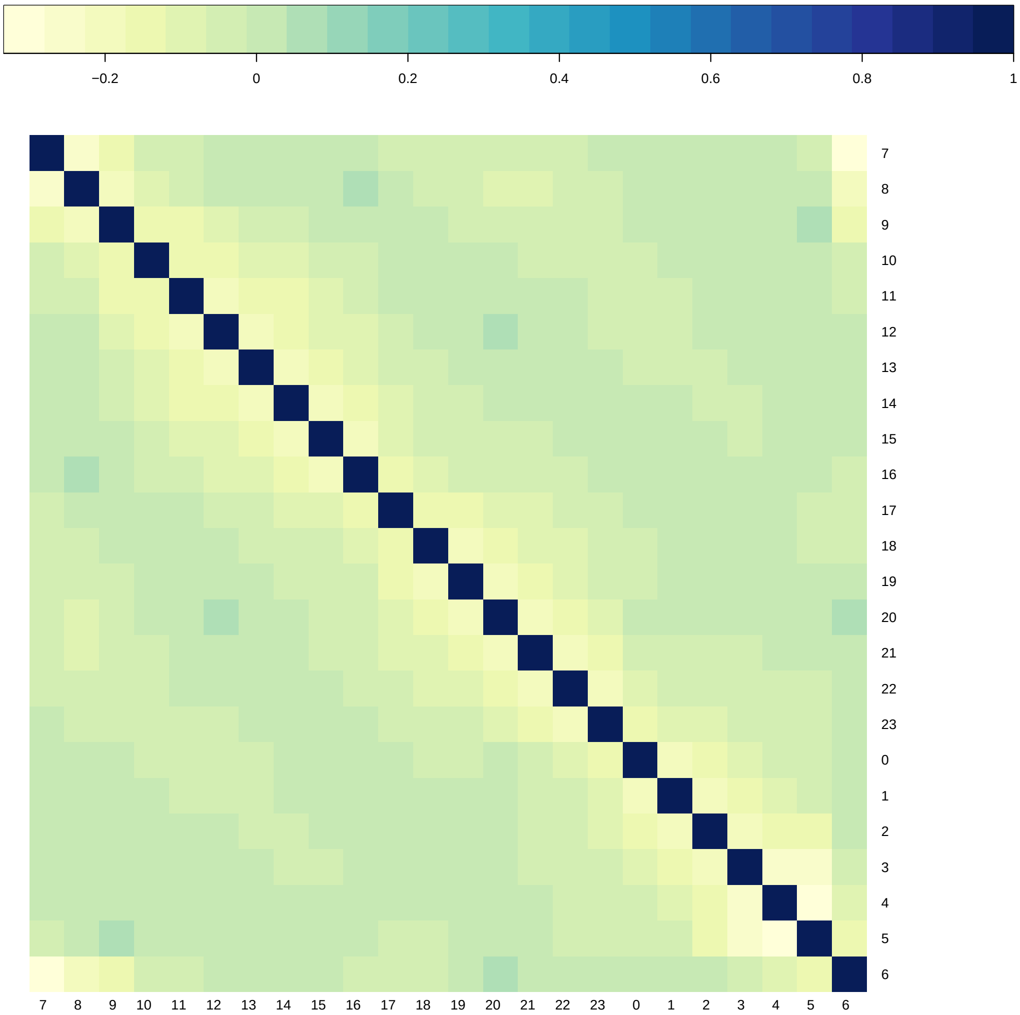


Figure S5: Mean of the posterior for the marginal standardized precision matrix. The labels indicate hour of the day in a 24-hour clock.

plot for the last 5% of times in the hold-out period and, again, reveals excellent agreement between the mean of the posterior predictive distribution and the test data, as well as narrow credible intervals.

### S5.2.3 Within-day filtering

For consistency with standard notation (see, for example Petris et al., 2009), in the following two sections we denote the observation and state equation as

$$\boldsymbol{y}_t = F\boldsymbol{\eta}_t + \boldsymbol{\epsilon}_t, \qquad \boldsymbol{\epsilon}_t \sim \mathrm{N}_p(\boldsymbol{0}, V)$$

and

$$\boldsymbol{\eta}_t = G\boldsymbol{\eta}_{t-1} + \boldsymbol{\zeta}_t, \qquad \boldsymbol{\zeta}_t \sim \mathrm{N}_k(\boldsymbol{0}, W).$$

Therefore, for the gas demand application, $\boldsymbol{y}_t$ represents mean-centered gas demand $\boldsymbol{y}_t - \boldsymbol{\mu}_t$, $F = \Lambda$, $G = \Gamma$, $V = \Sigma$, $W = \Pi$ and $\boldsymbol{\eta}_0 \sim \mathrm{N}_k(\boldsymbol{0}, I_k)$.

Let $\boldsymbol{y}_{s:t}$ denote the collection of vectors $(\boldsymbol{y}_s, \ldots, \boldsymbol{y}_t)$ and let $\boldsymbol{y}_{t,g:h}$ denote the subvector $(y_{t,g}, \ldots, y_{t,h})^{\mathrm{T}}$. Then at hour $h-1$ of day $t$, we write the filtering distribution as

$$\boldsymbol{\eta}_t | \boldsymbol{y}_{1:(t-1)}, \boldsymbol{y}_{t,1:(h-1)} \sim \mathrm{N}_k(\boldsymbol{m}_t^{(h-1)}, C_t^{(h-1)})$$

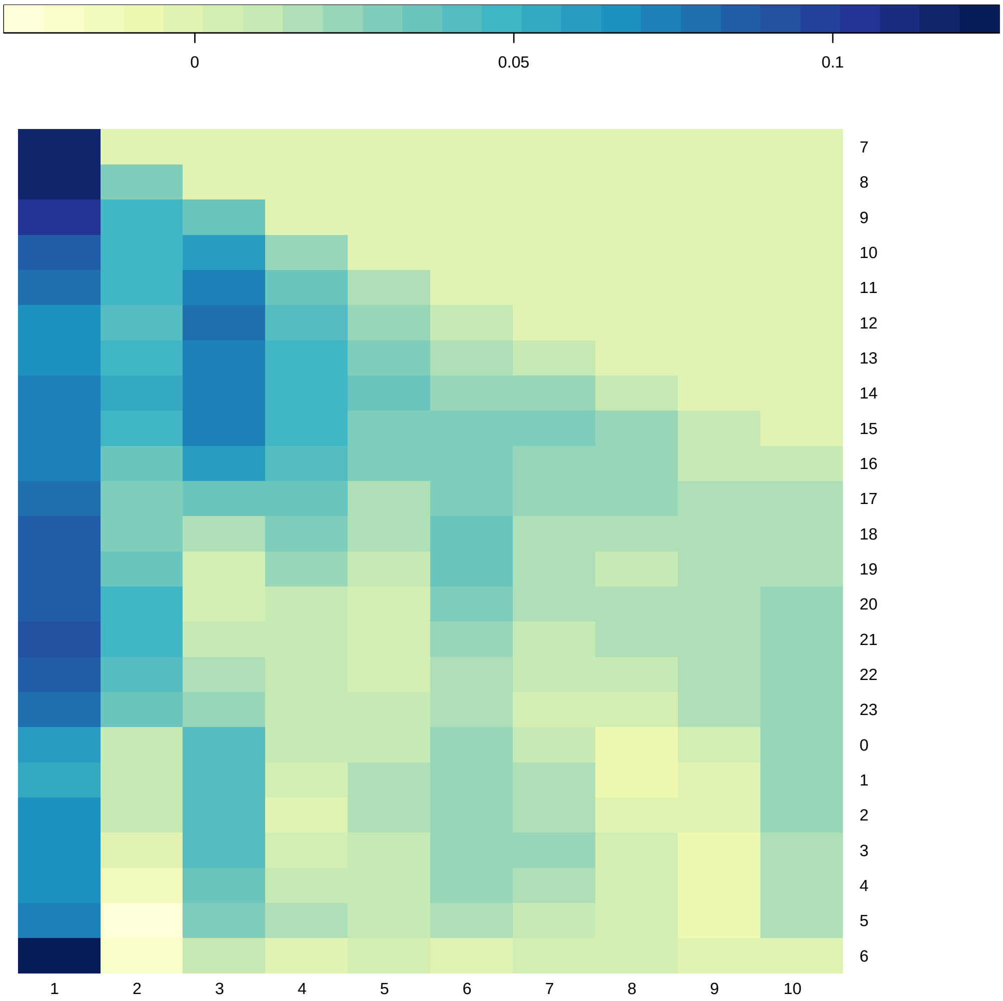


Figure S6: Mean of the posterior for the identified factor loadings matrix $\tilde{\Lambda}$. The labels on the right vertical axis indicate hour of the day in a 24-hour clock.

for $h = 2, \ldots, p$, noting that when $h = 1$, the corresponding distribution is

$$\boldsymbol{\eta}_{t-1}|\boldsymbol{y}_{1:(t-1)} \sim \mathrm{N}_k(\boldsymbol{m}_{t-1}^{(p)}, C_{t-1}^{(p)})$$

so that $\boldsymbol{m}_t^{(0)} = \boldsymbol{m}_{t-1}^{(p)}$ and $C_t^{(0)} = C_{t-1}^{(p)}$.

At hour $h$ of day $t$, we then:

1. Perform a prediction step if $h = 1$ by calculating

$$\begin{aligned} \boldsymbol{a}_t &= E(\boldsymbol{\eta}_t|\boldsymbol{y}_{1:(t-1)}) = G\boldsymbol{m}_{t-1}^{(p)} \\ R_t &= \mathrm{Var}(\boldsymbol{\eta}_t|\boldsymbol{y}_{1:(t-1)}) = GC_{t-1}^{(p)}G^{\mathrm{T}} + W \end{aligned}$$

   and then

$$\begin{aligned} \boldsymbol{f}_t^{(0)} &= E(\boldsymbol{y}_t|\boldsymbol{y}_{1:(t-1)}) = F\boldsymbol{a}_t \\ Q_t^{(0)} &= \mathrm{Var}(\boldsymbol{y}_t|\boldsymbol{y}_{1:(t-1)}) = FR_tF^{\mathrm{T}} + V \\ B_t^{(0)} &= \mathrm{Cov}(\boldsymbol{\eta}_t, \boldsymbol{y}_t|\boldsymbol{y}_{1:(t-1)}) = R_tF^{\mathrm{T}}. \end{aligned}$$

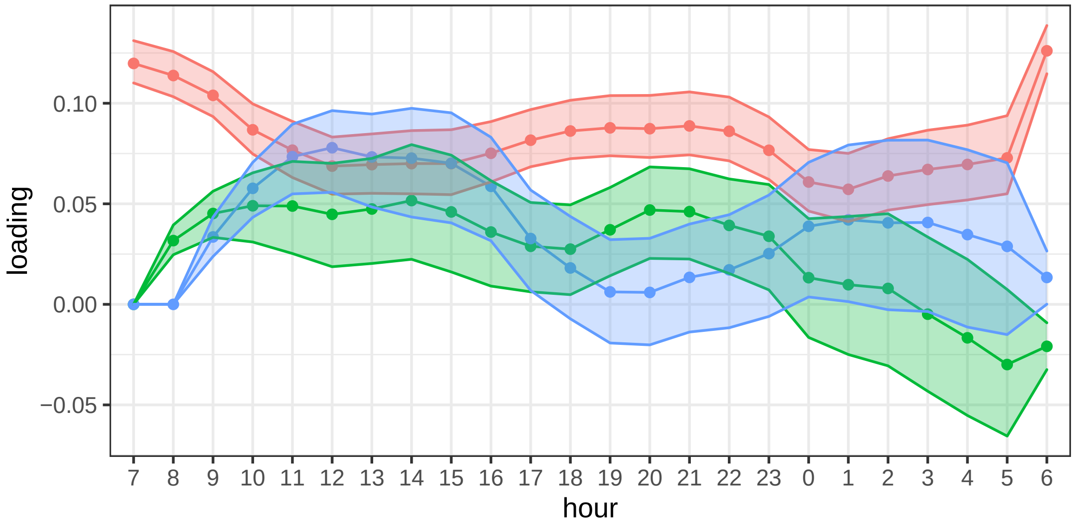


Figure S7: Summaries of the marginal posterior densities for the non-zero loadings of the first three factors in the identified factor loadings matrix $\tilde{\Lambda}$. The densities for factor 1 (—), factor 2 (—) and factor 3 (—) are summarized through their means and 95% equi-tailed credible intervals.

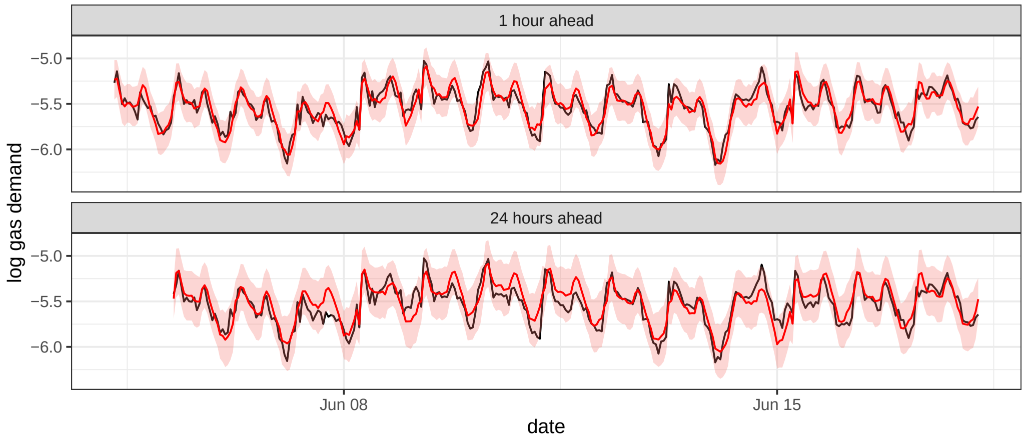


Figure S8: For the last 5% of times in the hold-out period, means (—) and 95% equi-tailed credible intervals ( ) for the one-step ahead and 24-step ahead posterior predictive distributions. The observed data are also shown (—).

We then construct

$$\boldsymbol{g}_t^{(0)\,\mathrm{T}} = (\boldsymbol{f}_t^{(0)\,\mathrm{T}}, \boldsymbol{a}_t^{\mathrm{T}})$$

and

$$S_t^{(0)} = \begin{pmatrix} Q_t^{(0)} & B_t^{(0)\,\mathrm{T}} \\ B_t^{(0)} & R_t \end{pmatrix}.$$

If $h > 1$, we will have available from the last prediction step $\boldsymbol{g}_t^{(h-1)}$ and $S_t^{(h)}$. Note that $\boldsymbol{g}_t^{(h)} = E\{(\boldsymbol{y}_{t,(h+1):p}^{\mathrm{T}}, \boldsymbol{\eta}_t^{\mathrm{T}})^{\mathrm{T}} | \boldsymbol{y}_{1:(t-1)}, \boldsymbol{y}_{t,1:h}\}$ is a $(k+p-h)$-vector and $S_t^{(h)} = \mathrm{Var}\{(\boldsymbol{y}_{t,(h+1):p}^{\mathrm{T}}, \boldsymbol{\eta}_t^{\mathrm{T}})^{\mathrm{T}} | \boldsymbol{y}_{1:(t-1)}, \boldsymbol{y}_{t,1:h}\}$ is a $(k+p-h) \times (k+p-h)$ matrix for $h = 0, \ldots, p-1$ which can be partitioned as

$$\boldsymbol{g}_t^{(h)\,\mathrm{T}} = (g_{t,1}^{(h)}, \boldsymbol{g}_{t,-1}^{(h)\,\mathrm{T}})$$

and

$$S_t^{(h)} = \begin{pmatrix} S_{t,1,1}^{(h)} & \boldsymbol{s}_{t,-1,1}^{(h)\,\mathrm{T}} \\ \boldsymbol{s}_{t,-1,1}^{(h)} & S_{t,-1,-1}^{(h)} \end{pmatrix}.$$

2. Perform an update step by using the rules of conditioning for multivariate normal distributions to calculate

$$\begin{aligned} \boldsymbol{g}_t^{(h)} &= \boldsymbol{g}_{t,-1}^{(h-1)} + \boldsymbol{s}_{t,-1,1}^{(h-1)}(y_{t,h} - g_{t,1}^{(h-1)})/S_{t,1,1}^{(h-1)} \\ S_t^{(h)} &= S_{t,-1,-1}^{(h-1)} - \boldsymbol{s}_{t,-1,1}^{(h-1)}\boldsymbol{s}_{t,-1,1}^{(h-1)\,\mathrm{T}}/S_{t,1,1}^{(h-1)} \end{aligned}$$

and then

$$\begin{aligned} \boldsymbol{m}_t^{(h)} &= E(\boldsymbol{\eta}_t|\boldsymbol{y}_{1:(t-1)}, \boldsymbol{y}_{t,1:h}) = \boldsymbol{g}_{t,(p-h+1):(k+p-h)}^{(h)} \\ C_t^{(h)} &= \mathrm{Var}(\boldsymbol{\eta}_t|\boldsymbol{y}_{1:(t-1)}, \boldsymbol{y}_{t,1:h}) = S_{t,(p-h+1):(k+p-h),(p-h+1):(k+p-h)}^{(h)}. \end{aligned}$$

If $h < p$ it is also useful for the forecasting recursions (see next section) to note the within-day forecast means and variances

$$\begin{aligned} \boldsymbol{f}_t^{(h)} &= E(\boldsymbol{y}_{t,(h+1):p}|\boldsymbol{y}_{1:(t-1)}, \boldsymbol{y}_{t,1:h}) = \boldsymbol{g}_{t,1:(p-h)}^{(h)} \\ Q_t^{(h)} &= \mathrm{Var}(\boldsymbol{y}_{t,(h+1):p}|\boldsymbol{y}_{1:(t-1)}, \boldsymbol{y}_{t,1:h}) = S_{t,1:(p-h),1:(p-h)}^{(h)}. \end{aligned}$$

### S5.2.4 Within-day forecasting

Consider generating forecasts using the data up to and including hour $h$ of day $t$ using the output of the filtering algorithm at that time, namely $\boldsymbol{m}_t^{(h)}$, $C_t^{(h)}$, $\boldsymbol{f}_t^{(h)}$ and $Q_t^{(h)}$. For simplicity in presentation, the algorithm below characterizes the predictive distribution for forecasts that are 1 to $dp + h$ hours ahead where $d \geq 0$ can only take integer values and represents the number of days we wish to look into the future.

Denote $\boldsymbol{f}_t^{(h)}(\ell) = E(\boldsymbol{y}_{t+\ell}|\boldsymbol{y}_{1:(t-1)}, \boldsymbol{y}_{t,1:h})$ and $Q_t^{(h)}(\ell) = \mathrm{Var}(\boldsymbol{y}_{t+\ell}|\boldsymbol{y}_{1:(t-1)}, \boldsymbol{y}_{t,1:h})$ and then proceed as follows:

1. Set $\ell = 0$. If $h < p$, we define $\boldsymbol{f}_t^{(h)}(0) = (\boldsymbol{y}_{t,1:h}^{\mathrm{T}}, \boldsymbol{f}_t^{(h)\,\mathrm{T}})^{\mathrm{T}}$ and

$$Q_t^{(h)}(0) = \begin{pmatrix} 0 & 0 \\ 0 & Q_t^{(h)} \end{pmatrix}$$

since the first $h$ elements of $\boldsymbol{y}_t$ have already been observed. If $h = p$, we define $\boldsymbol{f}_t^{(p)}(0) = \boldsymbol{f}_{t+1}^{(0)} = F\boldsymbol{a}_t^{(p)}(0)$ where $\boldsymbol{a}_t^{(p)}(0) = G\boldsymbol{m}_t^{(p)}$ and $Q_t^{(p)}(0) = Q_{t+1}^{(0)} = FR_t^{(p)}(0)F^{\mathrm{T}} + V$ where $R_t^{(p)}(0) = GC_t^{(p)}G^{\mathrm{T}} + W$.

2. Then if $d > 0$:

   (a) If $h < p$, we initialize with $\boldsymbol{a}_t^{(h)}(0) = \boldsymbol{m}_t^{(h)}$ and $R_t^{(h)}(0) = C_t^{(h)}$. If $h = p$, we have already calculated $\boldsymbol{a}_t^{(p)}(0)$ and $R_t^{(p)}(0)$ in (1).

   (b) For $\ell = 1, \ldots, d$, we can then recursively calculate

$$\begin{aligned} \boldsymbol{a}_t^{(h)}(\ell) &= E(\boldsymbol{\eta}_{t+\ell}|\boldsymbol{y}_{1:(t-1)}, \boldsymbol{y}_{t,1:h}) = G\boldsymbol{a}_t^{(h)}(\ell-1) \\ R_t^{(h)}(\ell) &= \mathrm{Var}(\boldsymbol{\eta}_{t+\ell}|\boldsymbol{y}_{1:(t-1)}, \boldsymbol{y}_{t,1:h}) = GR_t^{(h)}(\ell-1)G^{\mathrm{T}} + W \end{aligned}$$

   and

$$\begin{aligned} \boldsymbol{f}_t^{(h)}(\ell) &= E(\boldsymbol{y}_{t+\ell}|\boldsymbol{y}_{1:(t-1)}, \boldsymbol{y}_{t,1:h}) = F\boldsymbol{a}_t^{(h)}(\ell) \\ Q_t^{(h)}(\ell) &= \mathrm{Var}(\boldsymbol{y}_{t+\ell}|\boldsymbol{y}_{1:(t-1)}, \boldsymbol{y}_{t,1:h}) = FR_t^{(h)}(\ell)F^{\mathrm{T}} + W. \end{aligned}$$

## References


Banerjee, S. and A. Roy (2014). *Linear Algebra and Matrix Analysis for Statistics.* Texts in Statistical Science. CRC Press.

Carter, C. K. and R. Kohn (1994). On Gibbs sampling for state space models. *Biometrika 81*(3), 541–553.

Frühwirth-Schnatter, S. (1994). Data augmentation and dynamic linear models. *Journal of Time Series Analysis 15*, 183–202.

Genz, A. and F. Bretz (2009). *Computation of Multivariate Normal and t Probabilities.* Lecture Notes in Statistics. Heidelberg: Springer-Verlag.

Genz, A., F. Bretz, T. Miwa, X. Mi, F. Leisch, F. Scheipl, and T. Hothorn (2021). *mvtnorm: Multivariate Normal and t Distributions.* R package version 1.1-2.

Gschlößl, S. and C. Czado (2008). Modelling count data with overdispersion and spatial effects. *Statistical Papers 49*, 531–552.

Gupta, A. K. and D. K. Nagar (2000). *Matrix Variate Distributions.* Boca Raton, Florida: Chapman & Hall/CRC.

Heaps, S. E. (2022). Enforcing stationarity through the prior in vector autoregressions. *J. Comput. Graph. Stat.*.

Heaps, S. E., M. Farrow, and K. J. Wilson (2020). Identifying the effect of public holidays on daily demand for gas. *J. R. Statist. Soc. A 183*(2), 471–492.

Hoff, P. D. (2009). Simulation of the matrix Bingham-von Mises-Fisher distribution, with applications to multivariate relational data. *J. Comput. Graph. Stat. 18*(2), 438–456.

Leung, D. and M. Drton (2016). Order-invariant prior specification in Bayesian factor analysis. *Stat. Probab. Lett. 111*, 60–66.

Muirhead, R. J. (2005). *Aspects of Multivariate Statistical Theory.* Hoboken, New Jersey: John Wiley and Sons.

Petris, G., S. Petrone, and P. Campagnoli (2009). *Dynamic Linear Models with R.* Springer-Verlag.

Seber, G. A. F. (2008). *A Matrix Handbook for Statisticians.* John Wiley & Sons.
